# Supplementary material for: Bayesian Uncertainty Quantification for Systems Biology Models Parameterized Using Qualitative Data
Source: arXiv:1909.00072 source file (2019-08-30)
Supplement: Supplementary file 1 [file SupplementaryInfo_compress.pdf]

**SUPPLEMENTARY INFORMATION**

# Bayesian Uncertainty Quantification for Systems Biology Models Parameterized Using Qualitative Data

Eshan D. Mitra, William S. Hlavacek

4 qualitative measurements

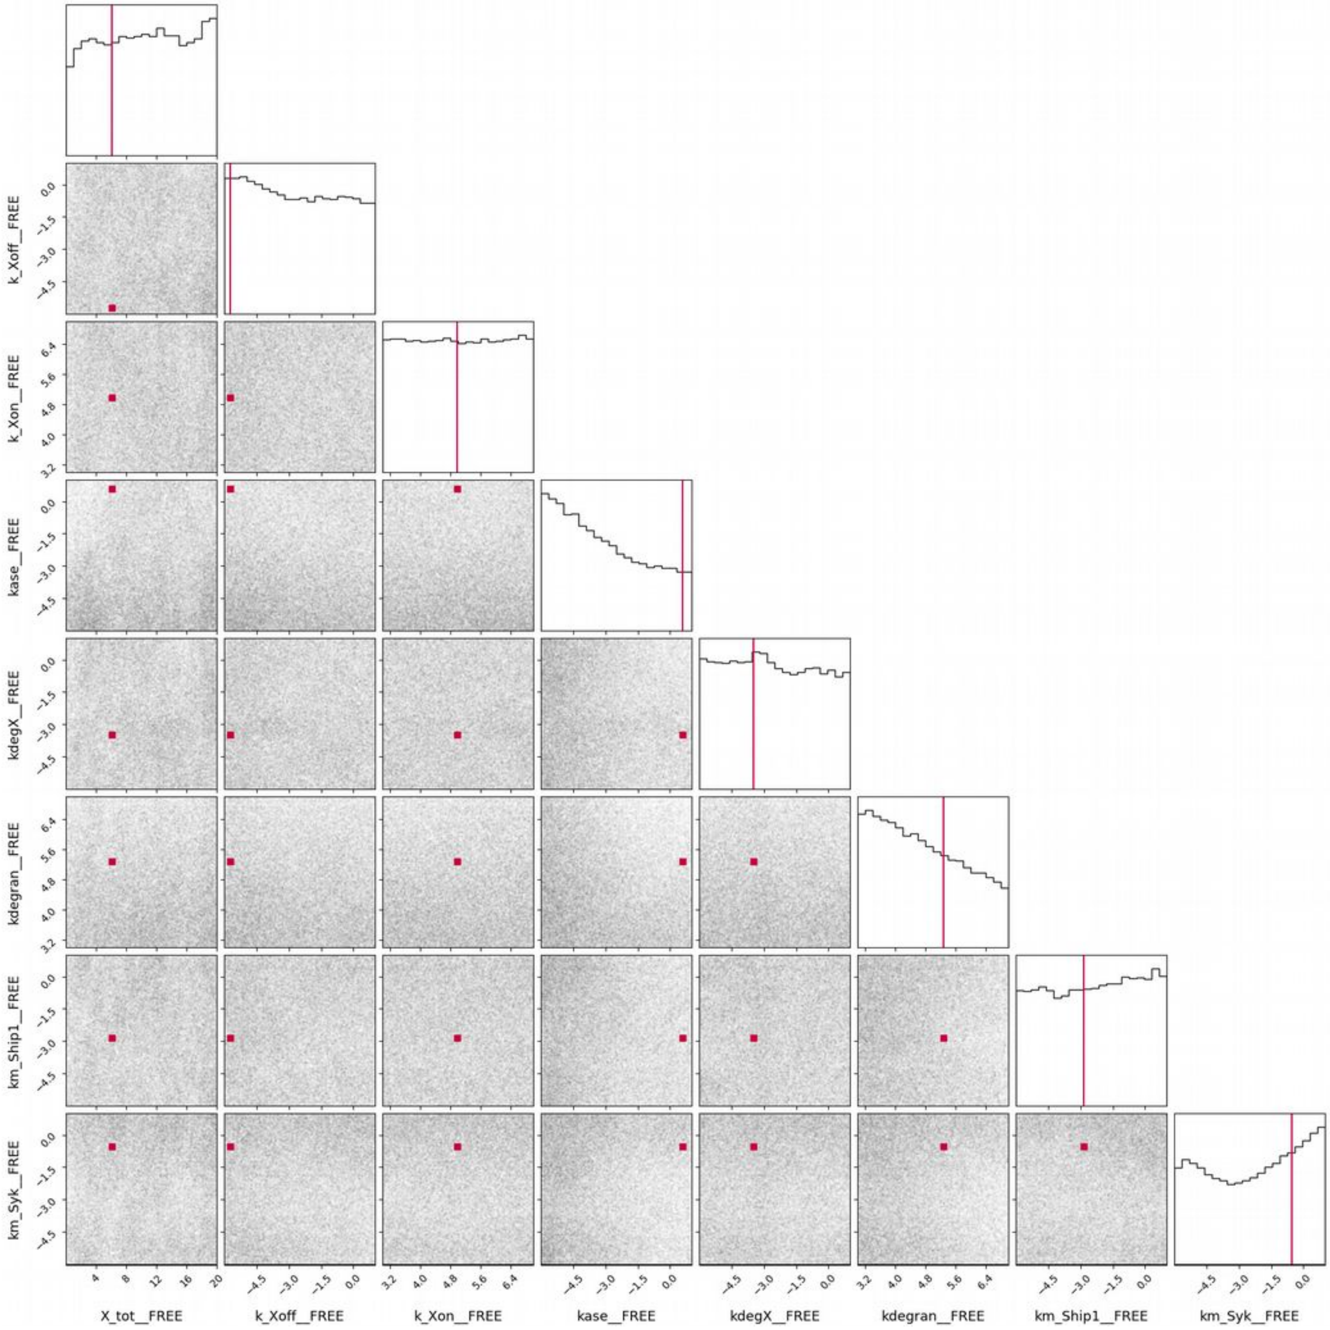

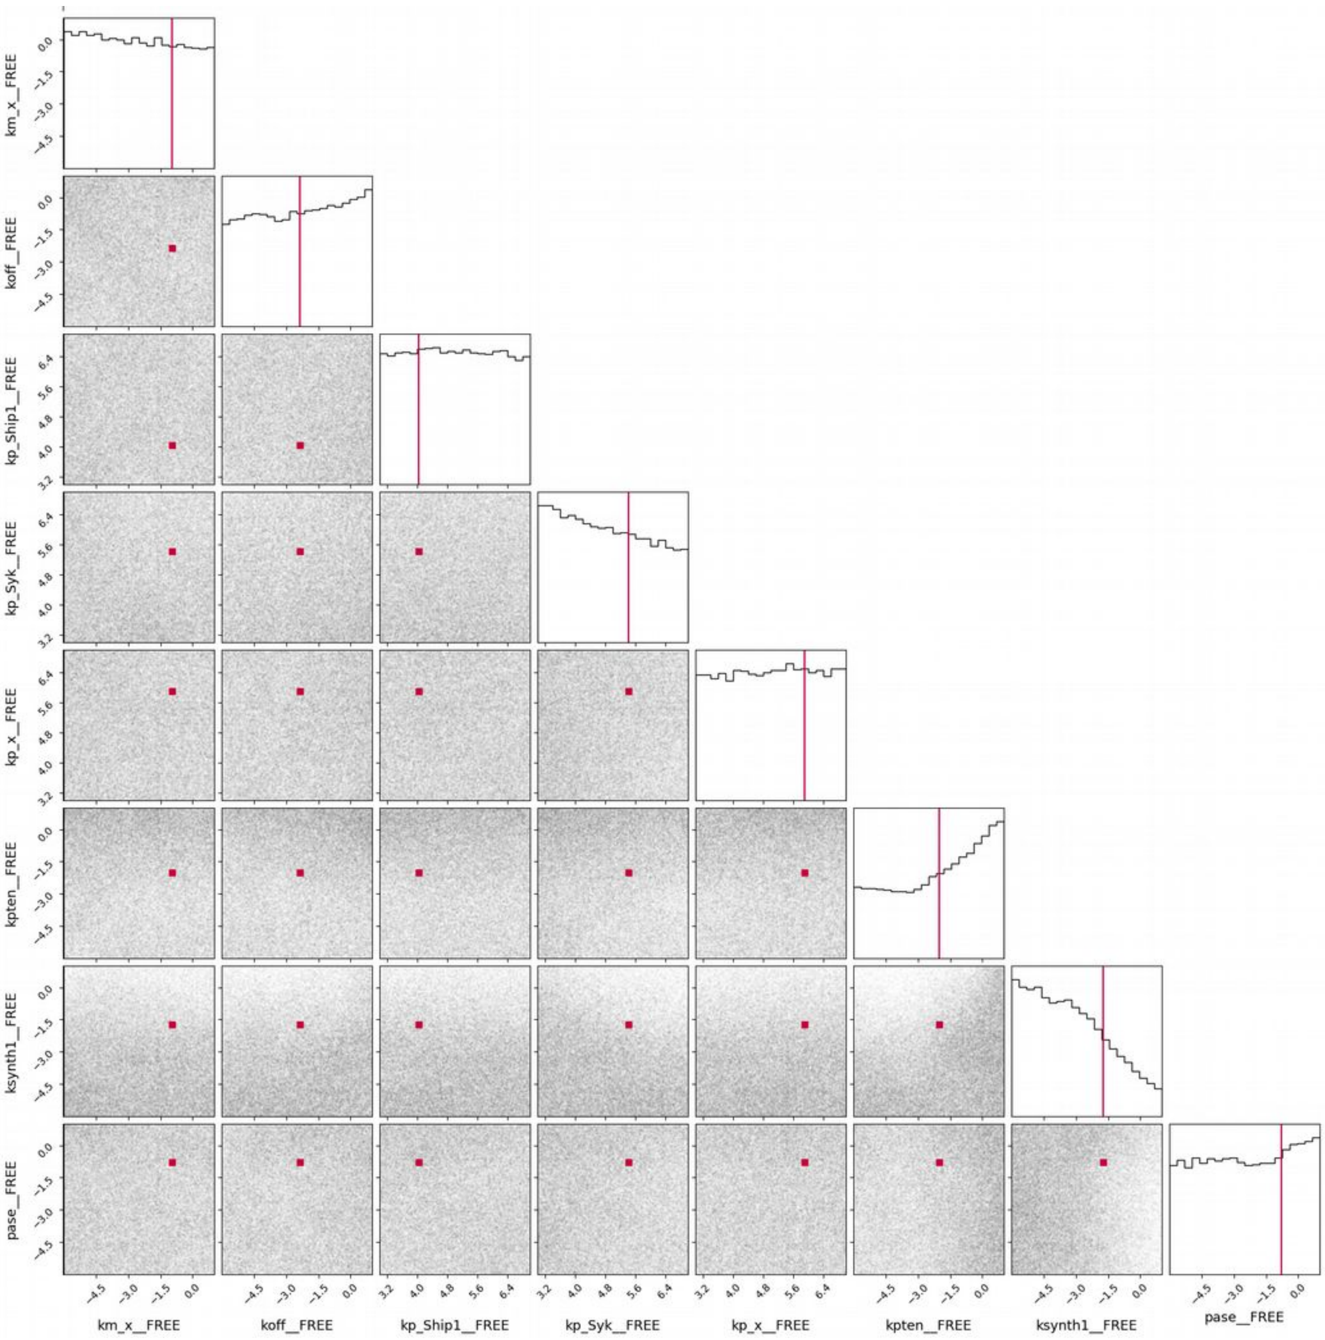

km_x__FREE
koff__FREE
kp_Ship1__FREE
kp_Syk__FREE
kp_x__FREE
kpten__FREE
ksynth1__FREE
pase__FREE

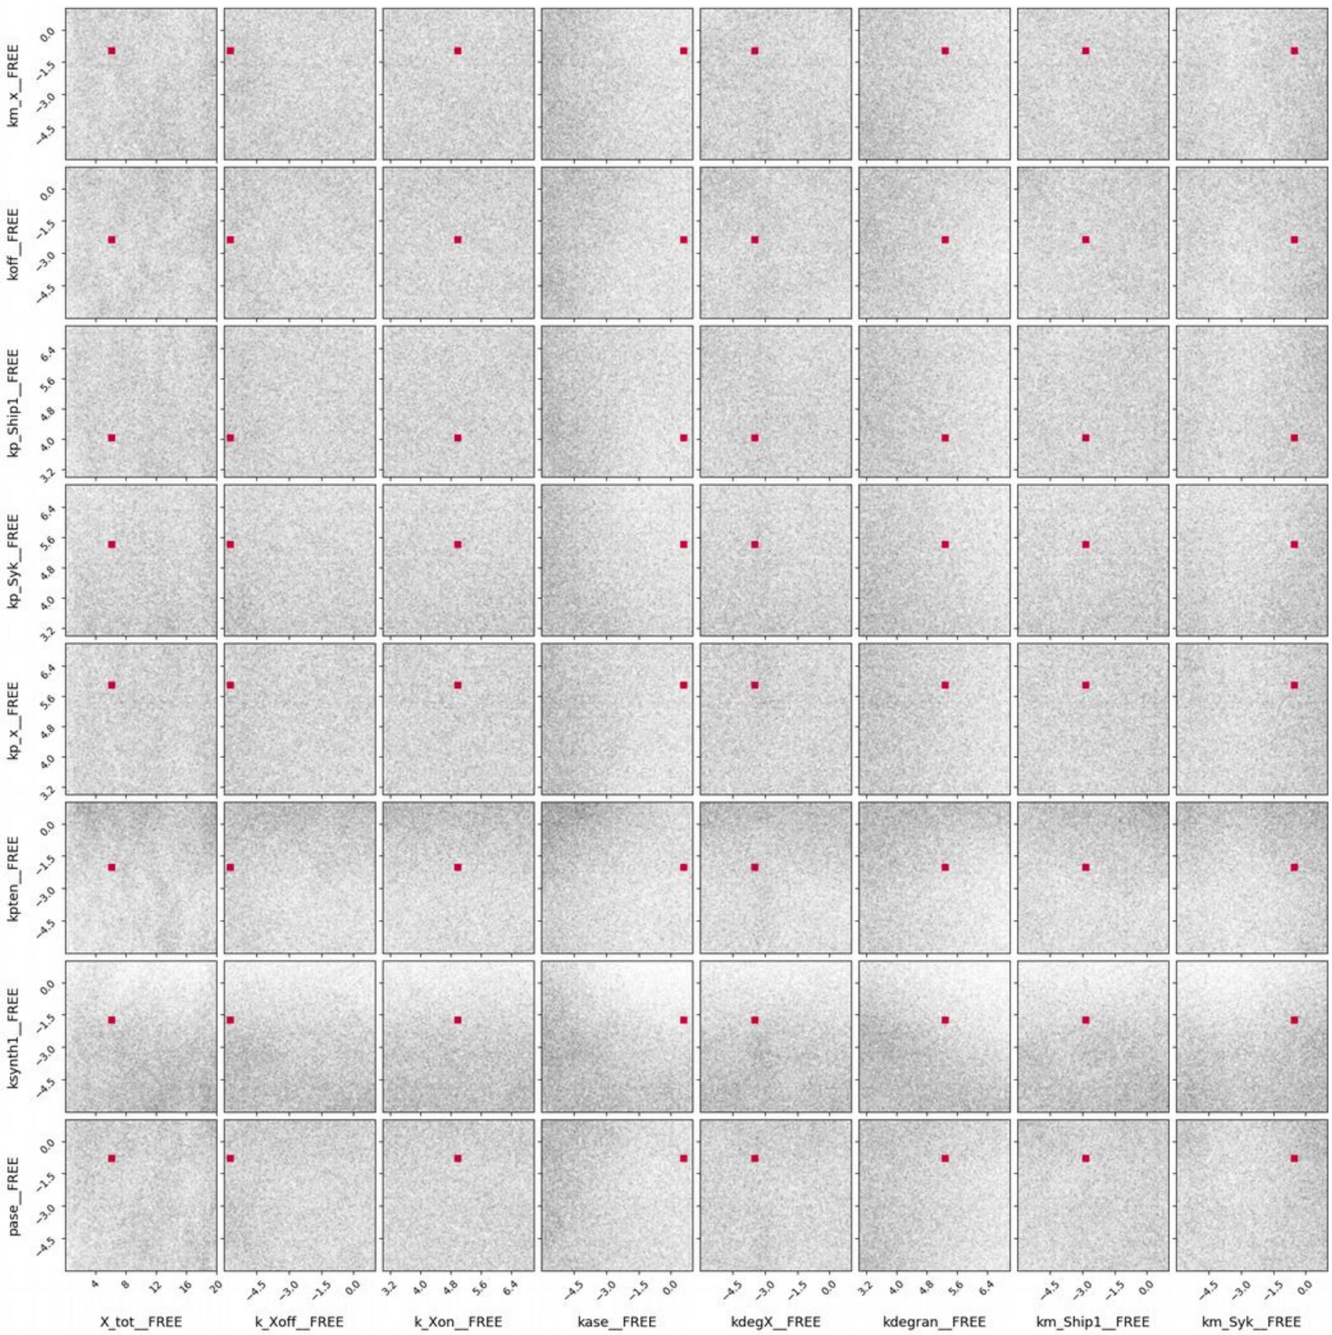


Figure S1: Corner plot showing the marginal posterior distribution for each pair of model parameters, under a measurement protocol consisting of 4 qualitative measurements, each with two possible categorical outcomes. The plot is split over the previous three pages for display purposes. Ground truth parameters are shown in red.

8 qualitative measurements

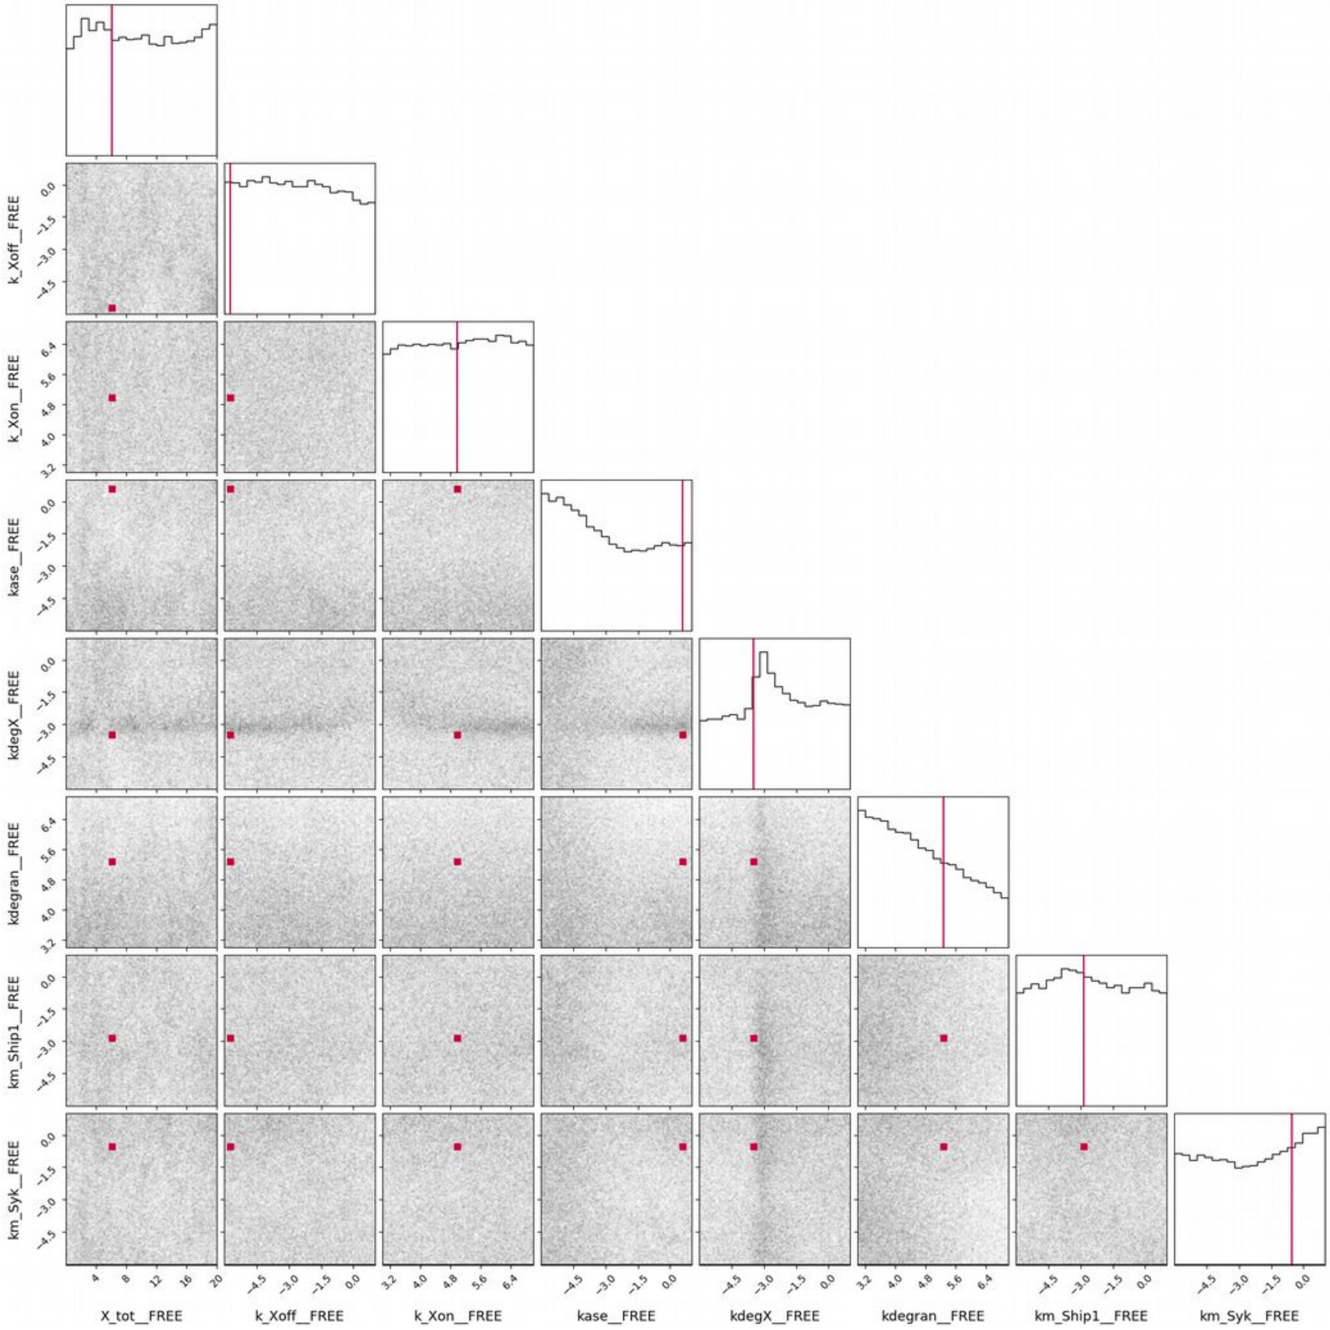

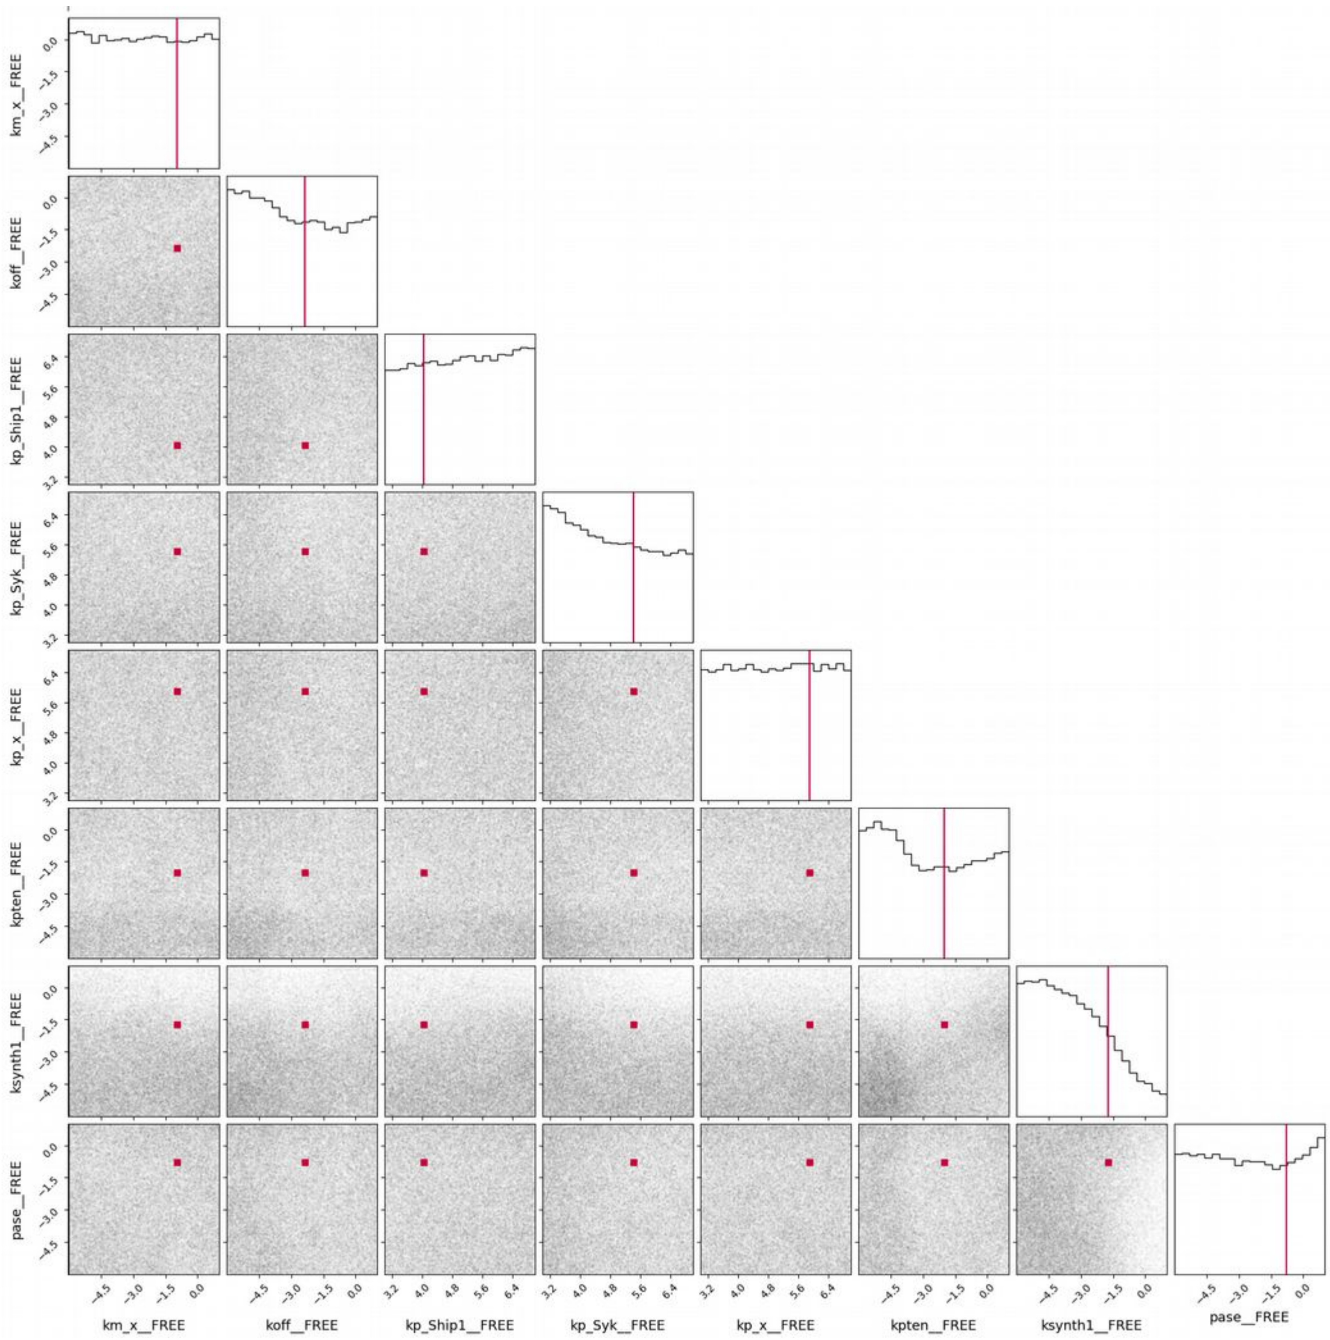
km_x__FREE
koff__FREE
kp_Ship1__FREE
kp_Syk__FREE
kp_x__FREE
kpten__FREE
ksynth1__FREE
pase__FREE

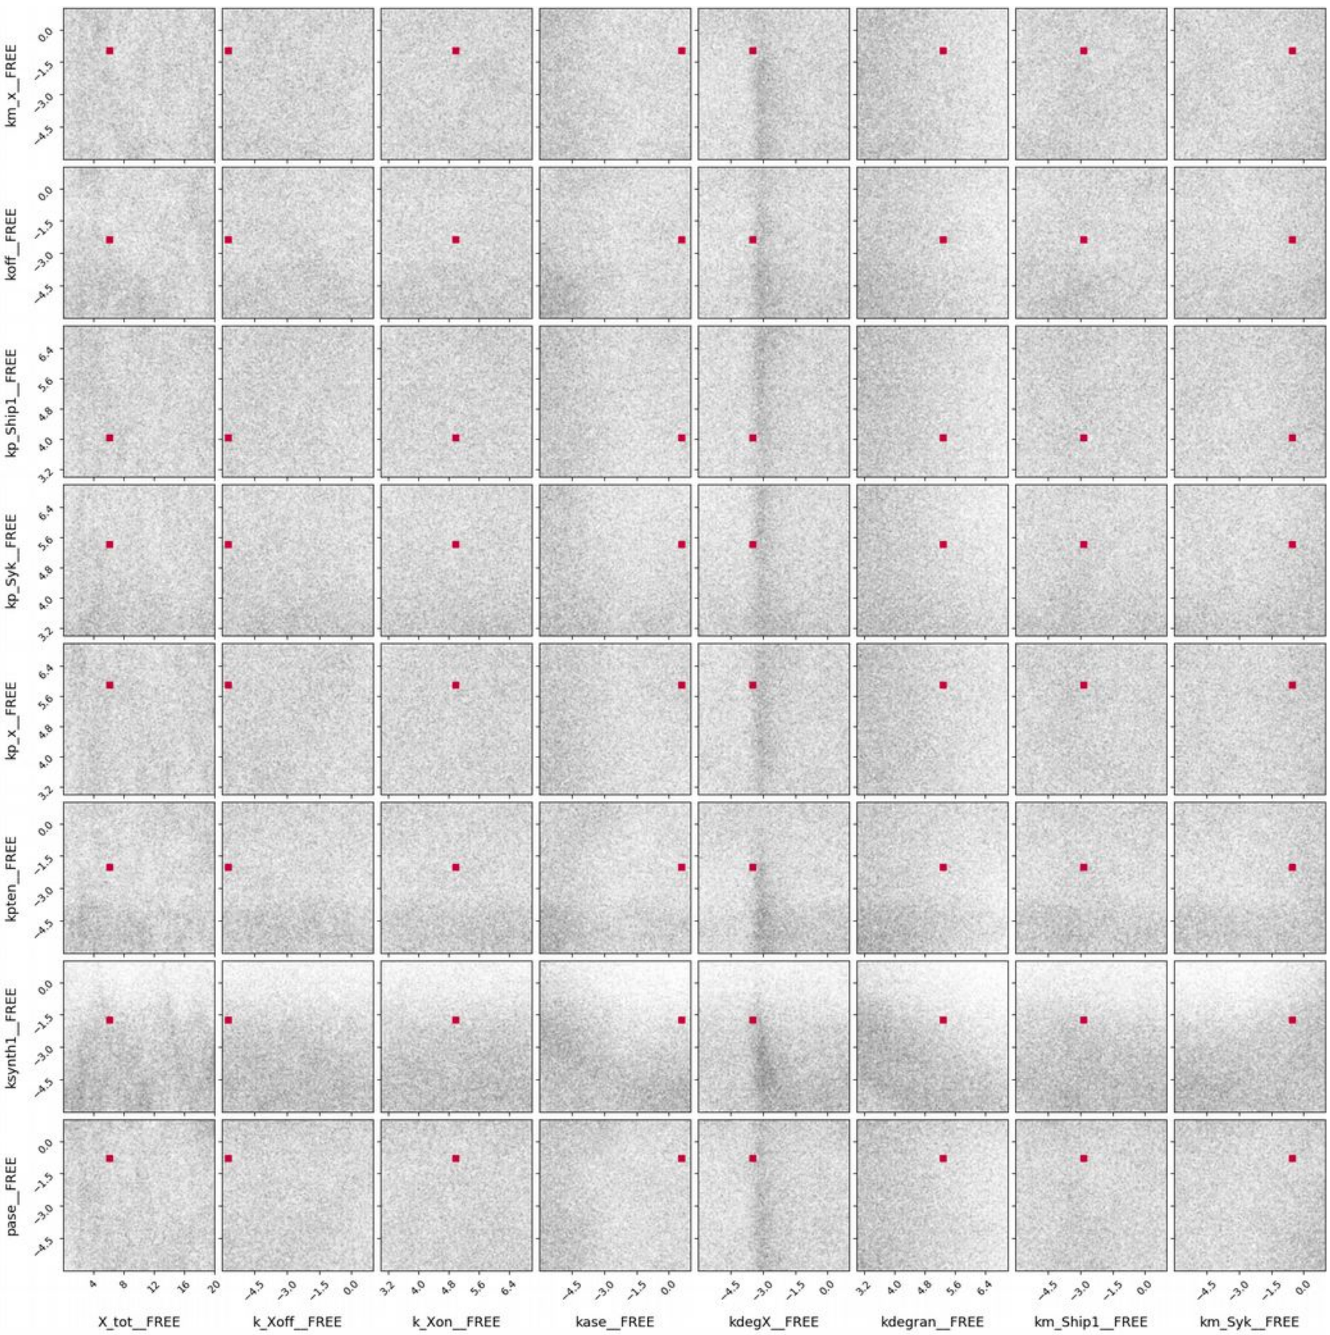


Figure S2: Corner plot showing the marginal posterior distribution for each pair of model parameters, under a measurement protocol consisting of 8 qualitative measurements, each with two possible categorical outcomes. The plot is split over the previous three pages for display purposes. Ground truth parameters are shown in red.

16 qualitative measurements

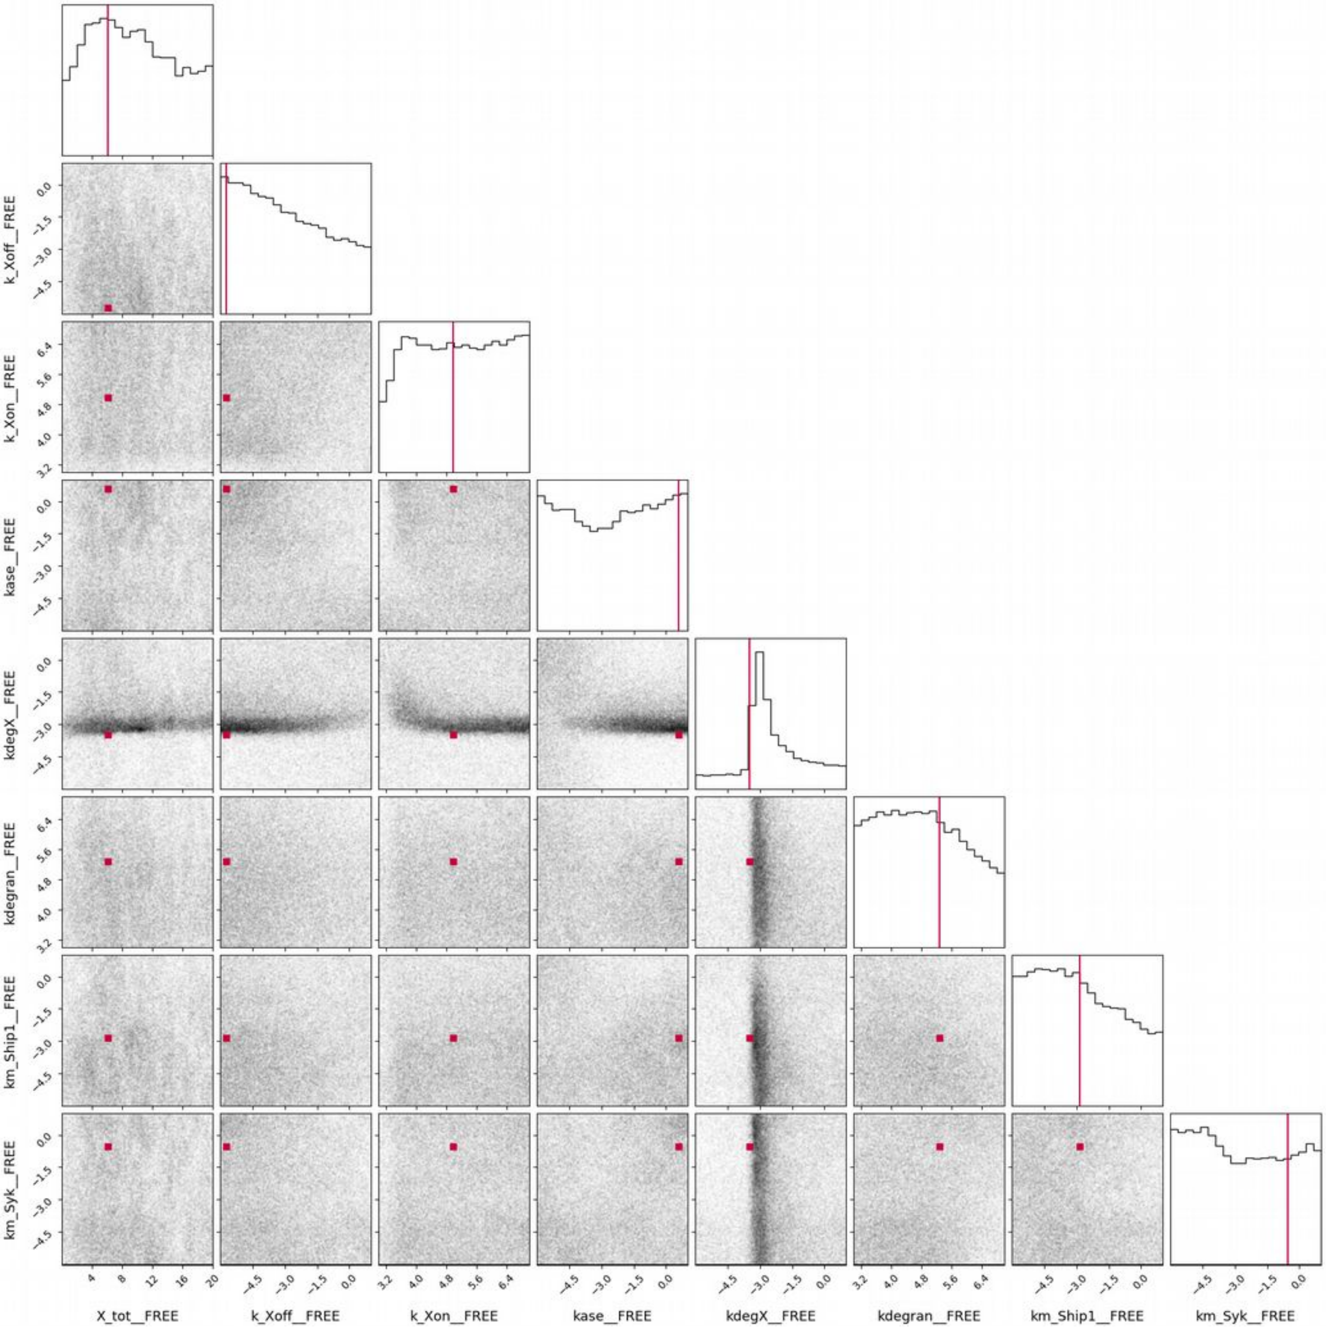

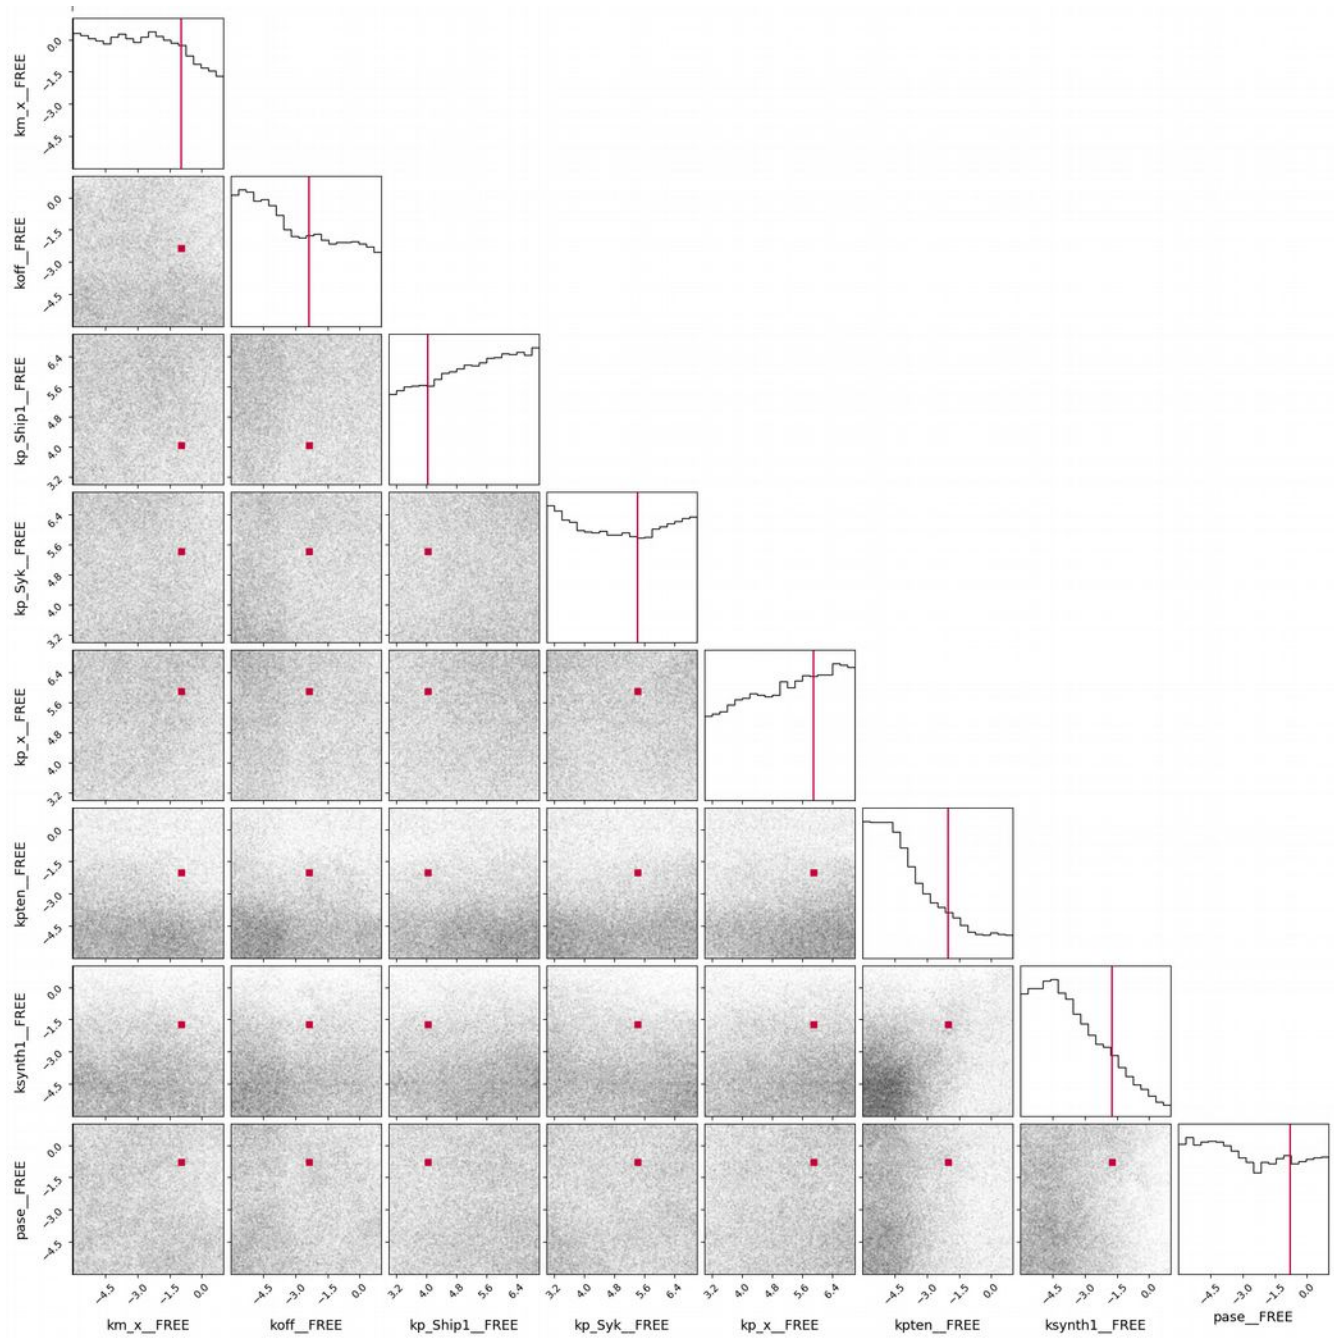
km_x__FREE
koff__FREE
kp_Ship1__FREE
kp_Syk__FREE
kp_x__FREE
kpten__FREE
ksynth1__FREE
pase__FREE

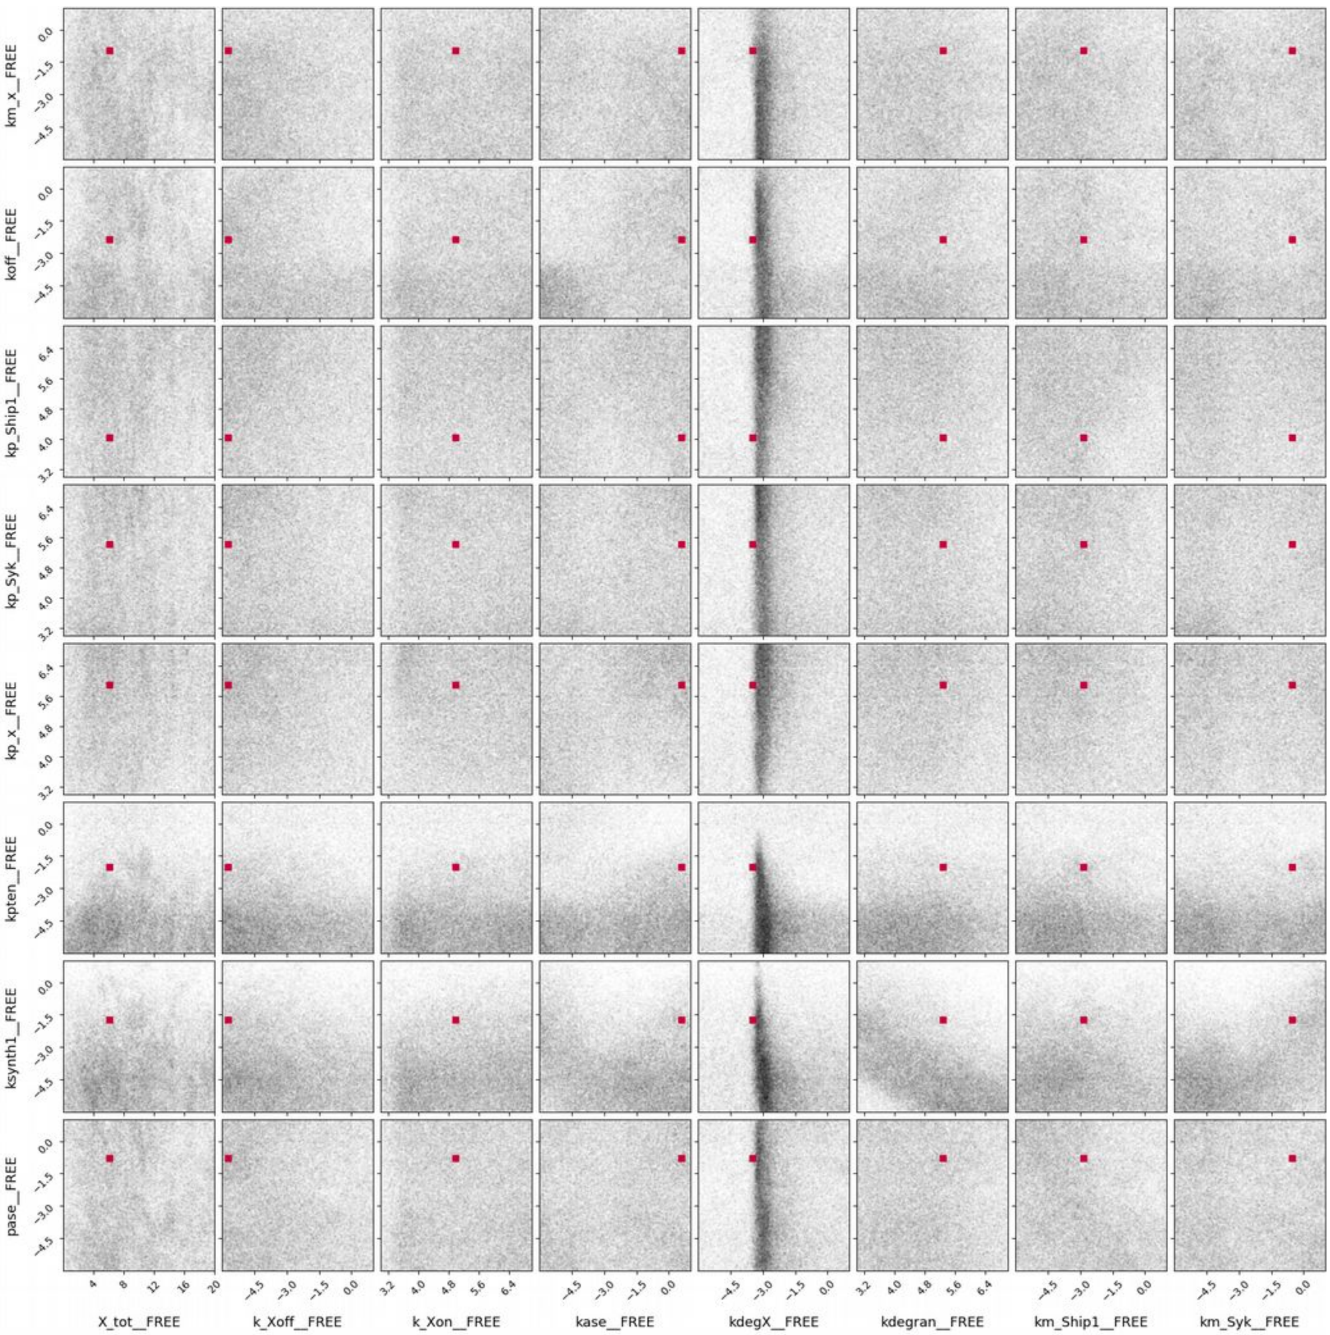


Figure S3: Corner plot showing the marginal posterior distribution for each pair of model parameters, under a measurement protocol consisting of 16 qualitative measurements, each with two possible categorical outcomes. The plot is split over the previous three pages for display purposes. Ground truth parameters are shown in red.

32 qualitative measurements

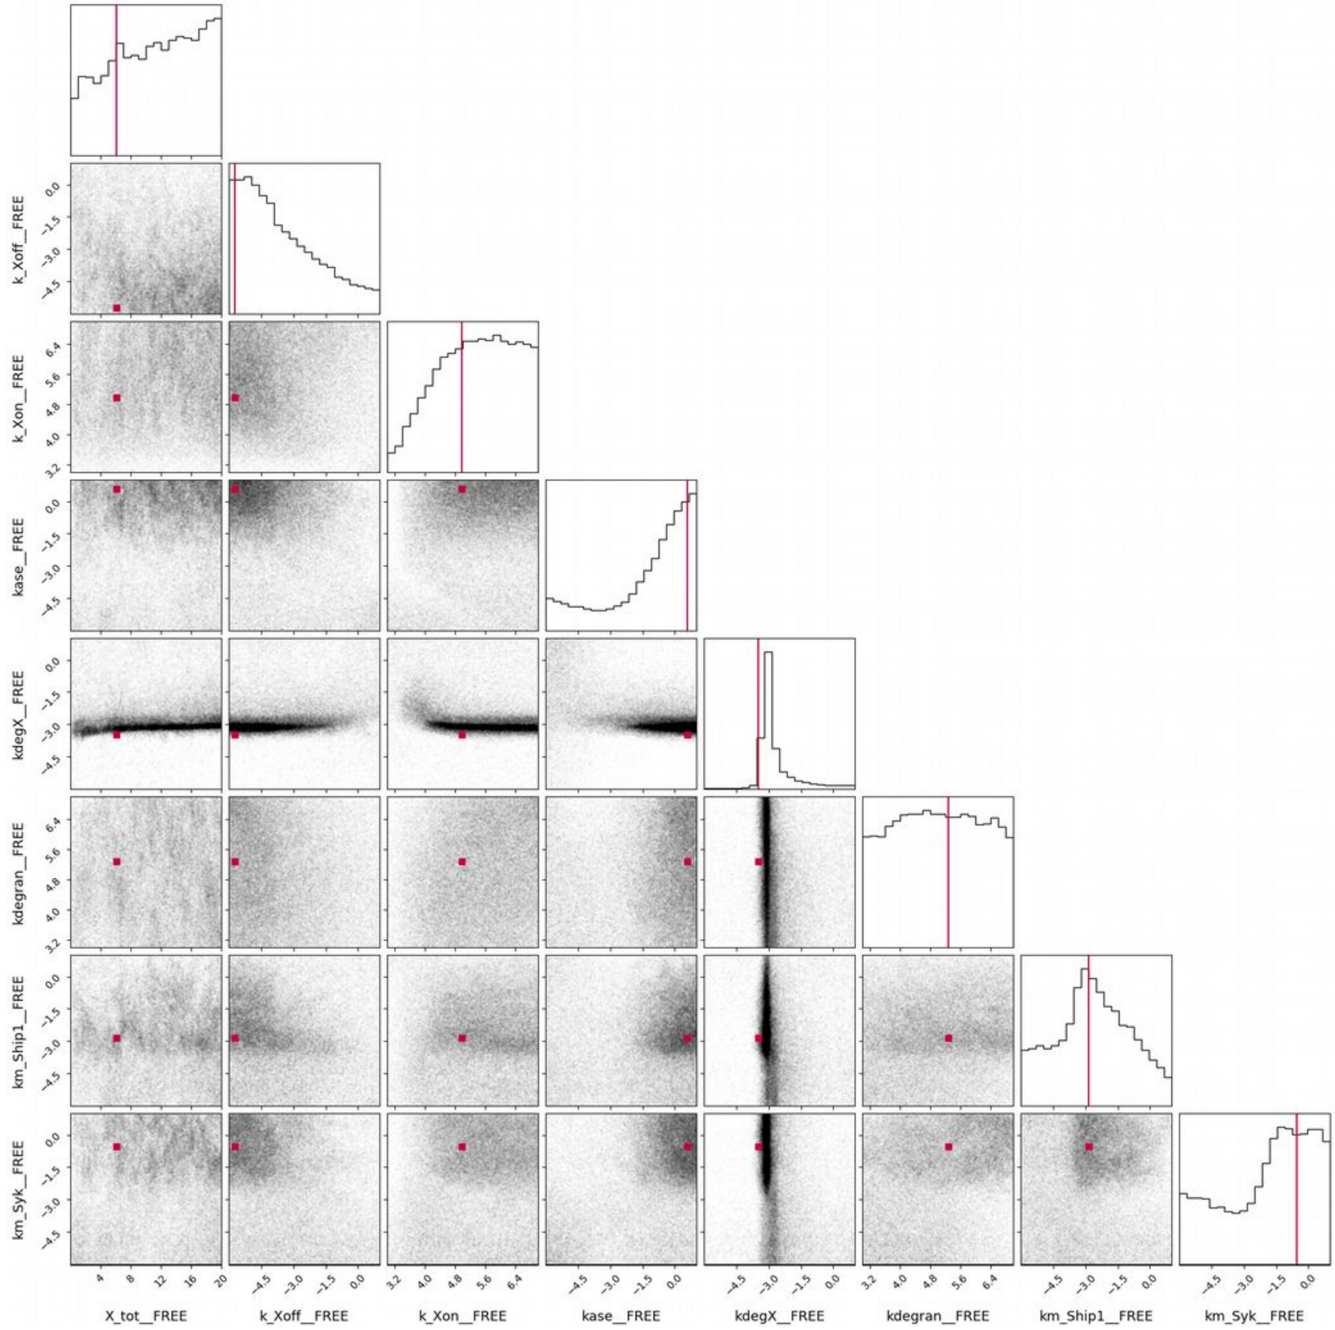

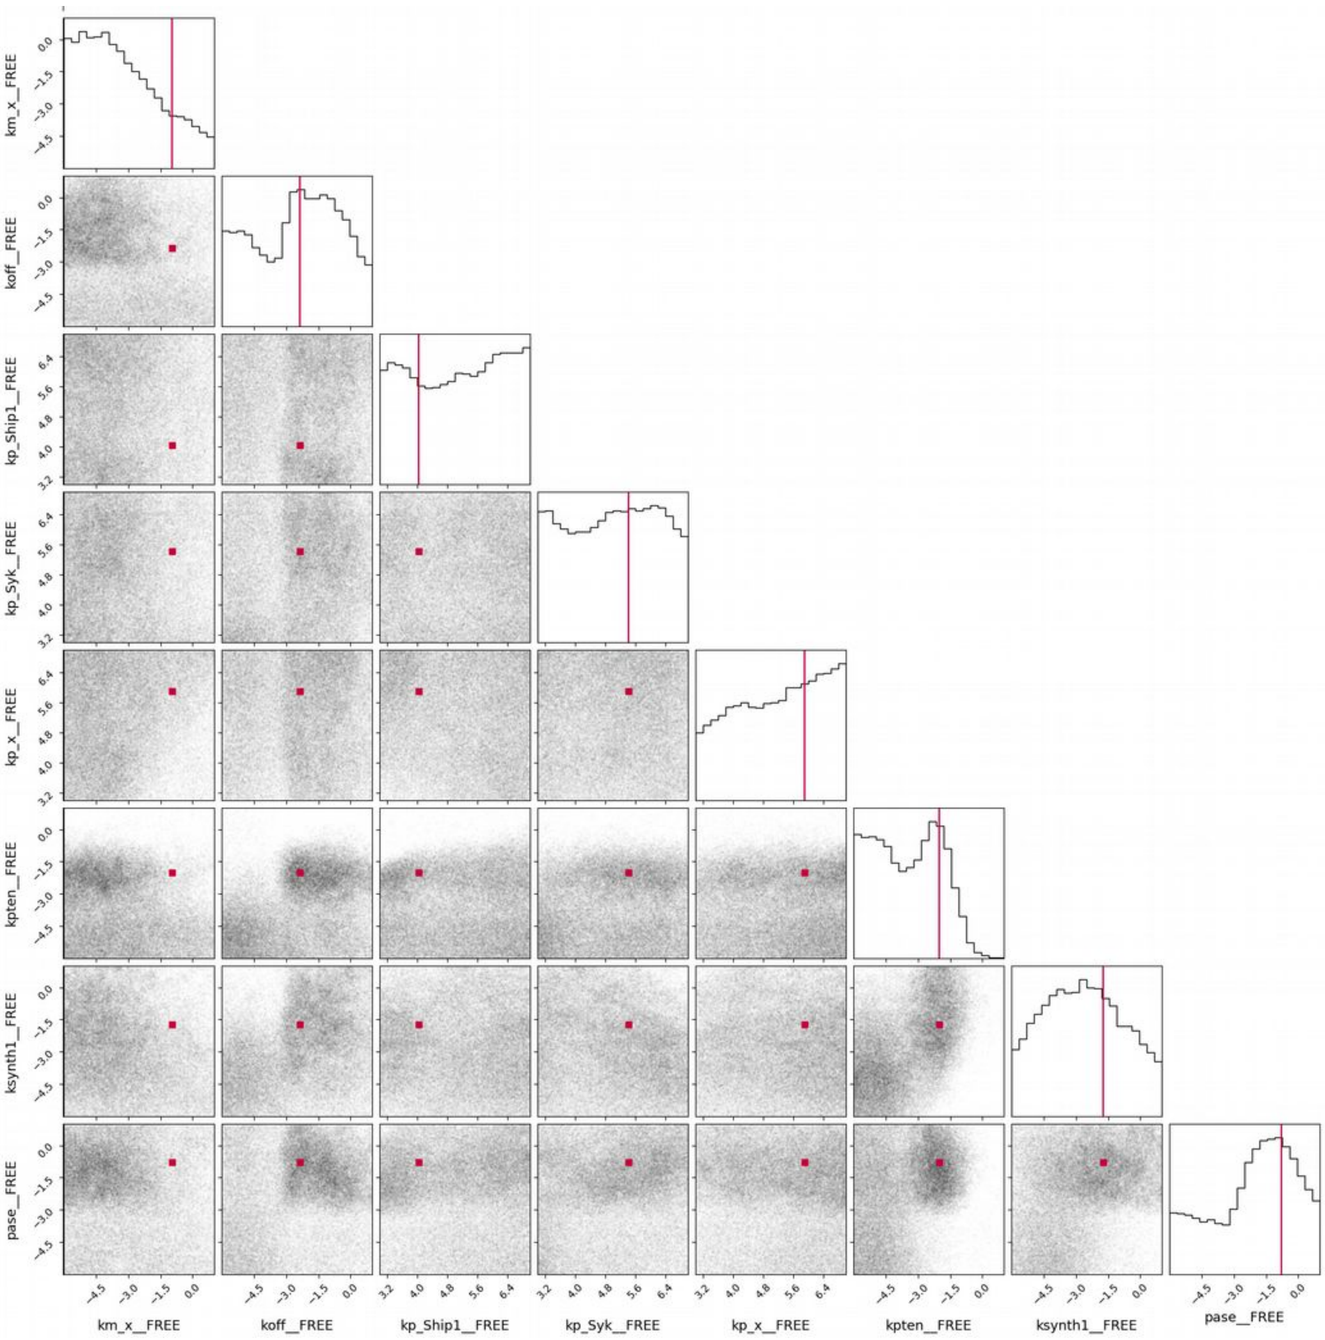

km_x__FREE
koff__FREE
kp_Ship1__FREE
kp_Syk__FREE
kp_x__FREE
kpten__FREE
ksynth1__FREE
pase__FREE

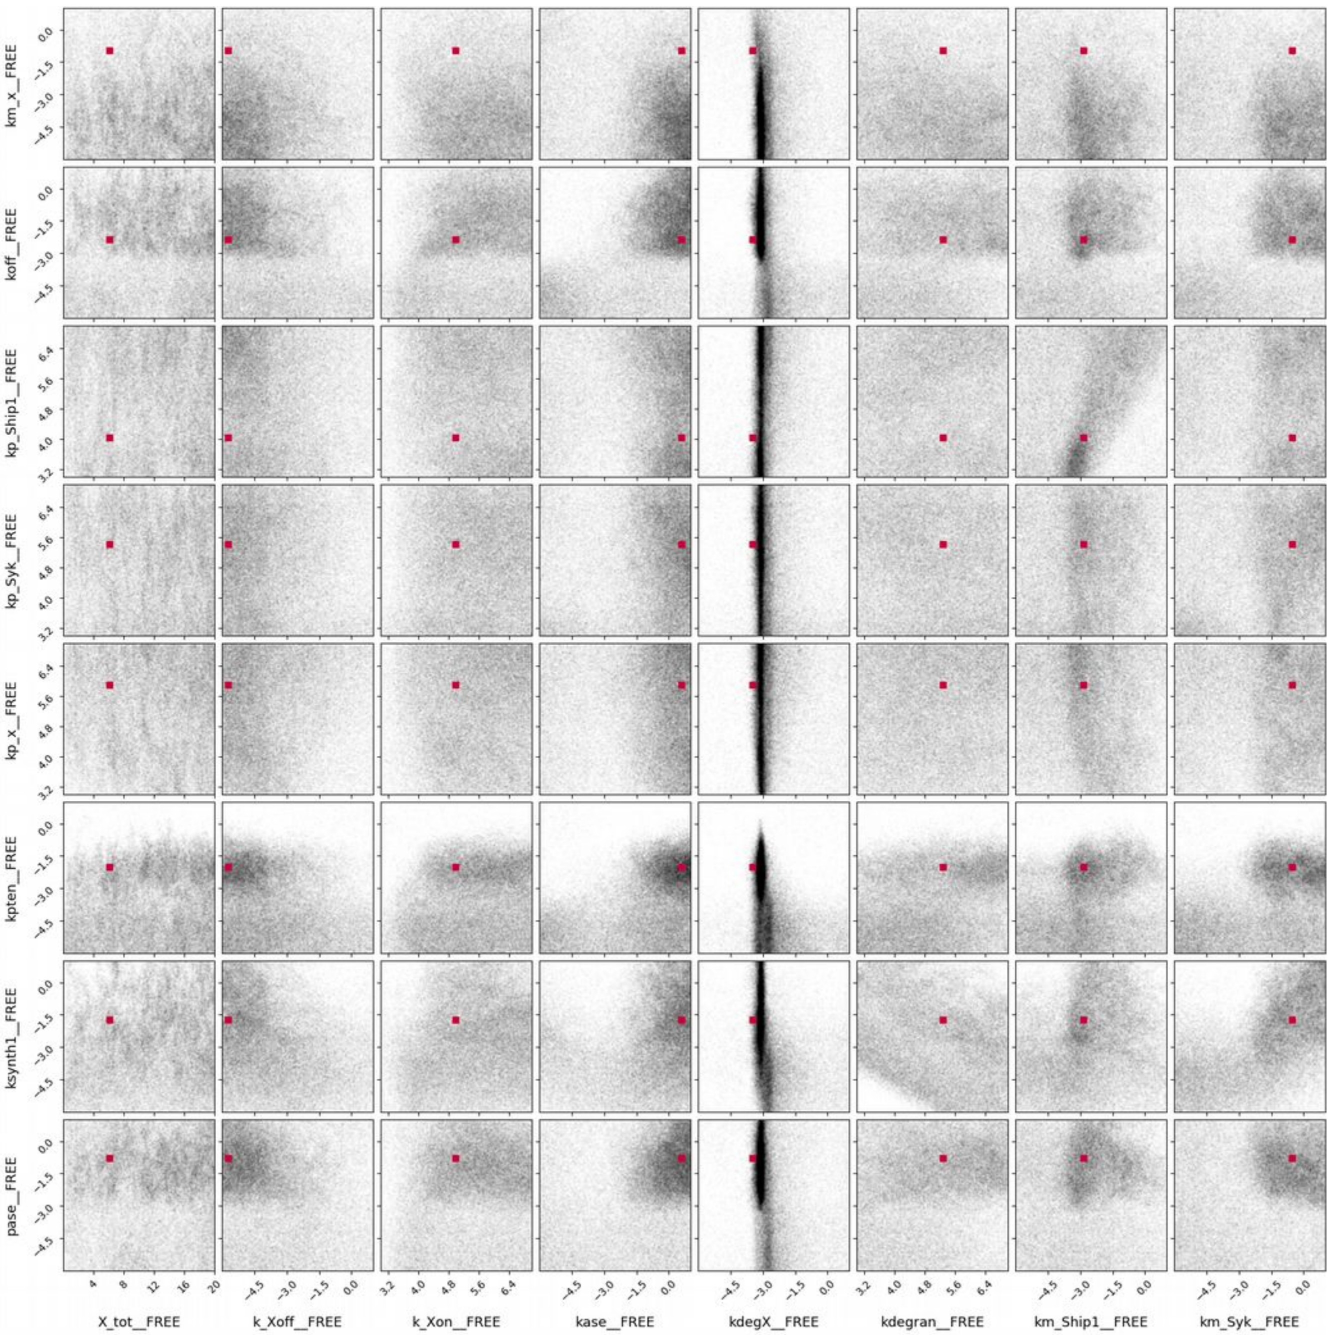


Figure S4: Corner plot showing the marginal posterior distribution for each pair of model parameters, under a measurement protocol consisting of 32 qualitative measurements, each with two possible categorical outcomes. The plot is split over the previous three pages for display purposes. Ground truth parameters are shown in red.

64 qualitative measurements

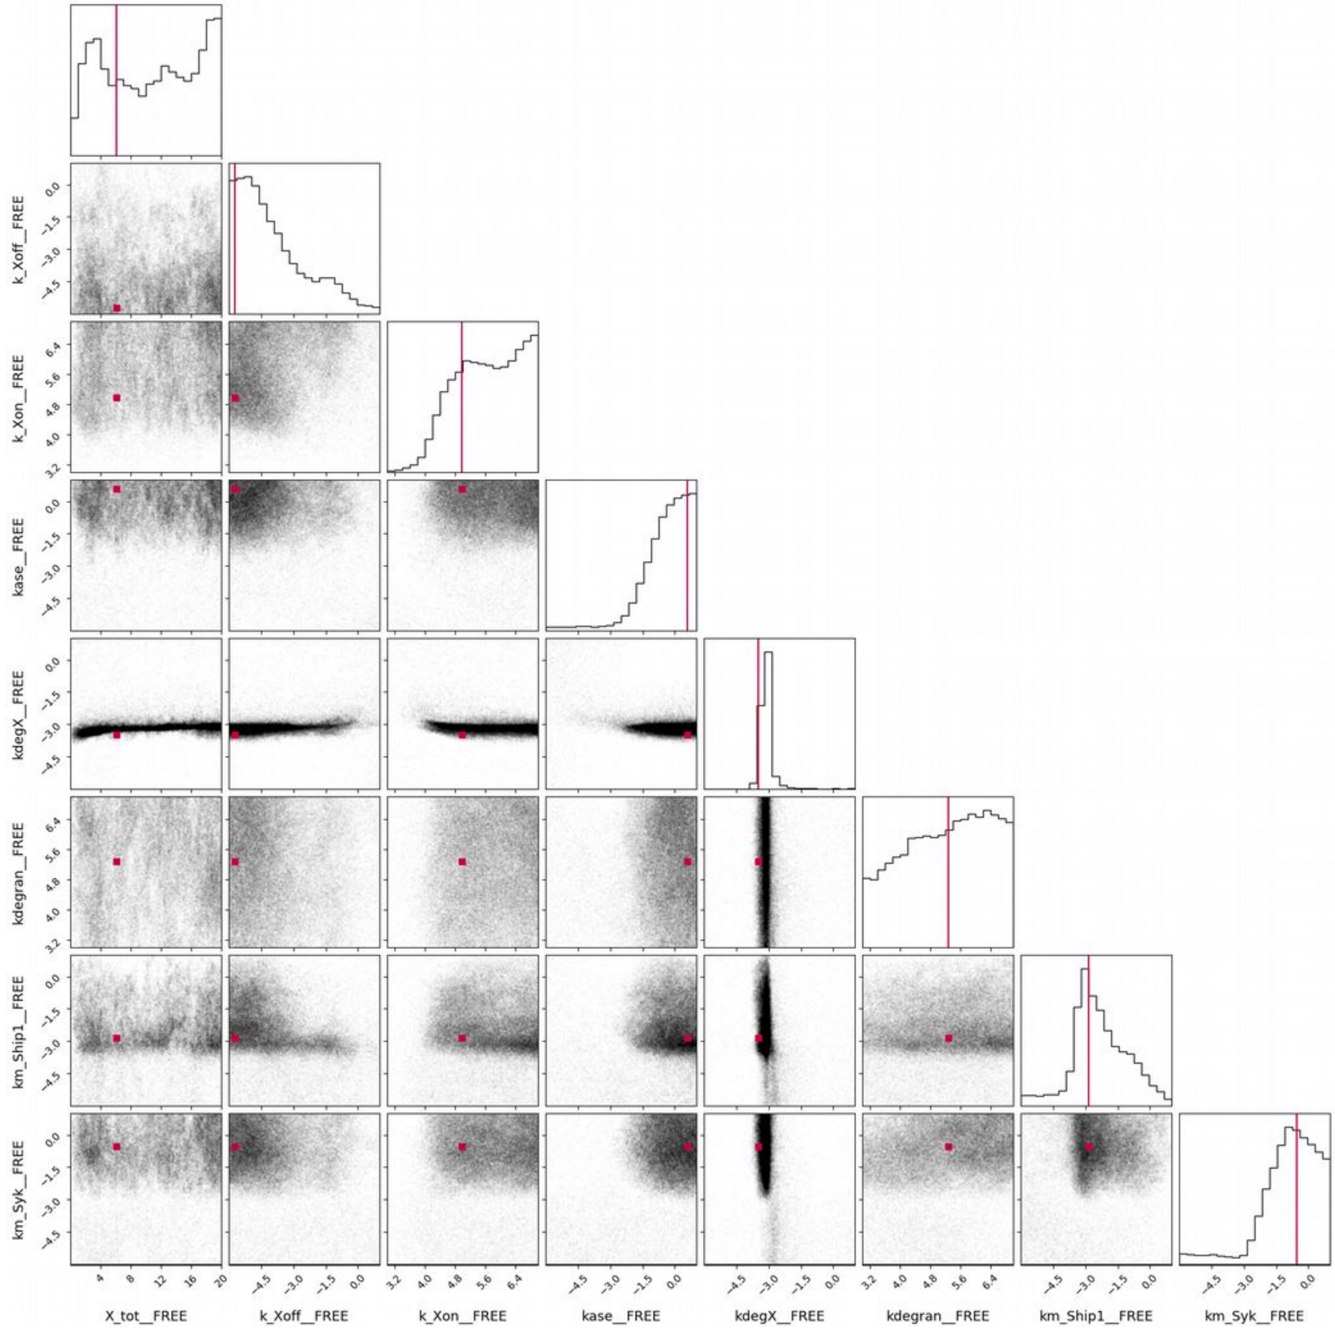

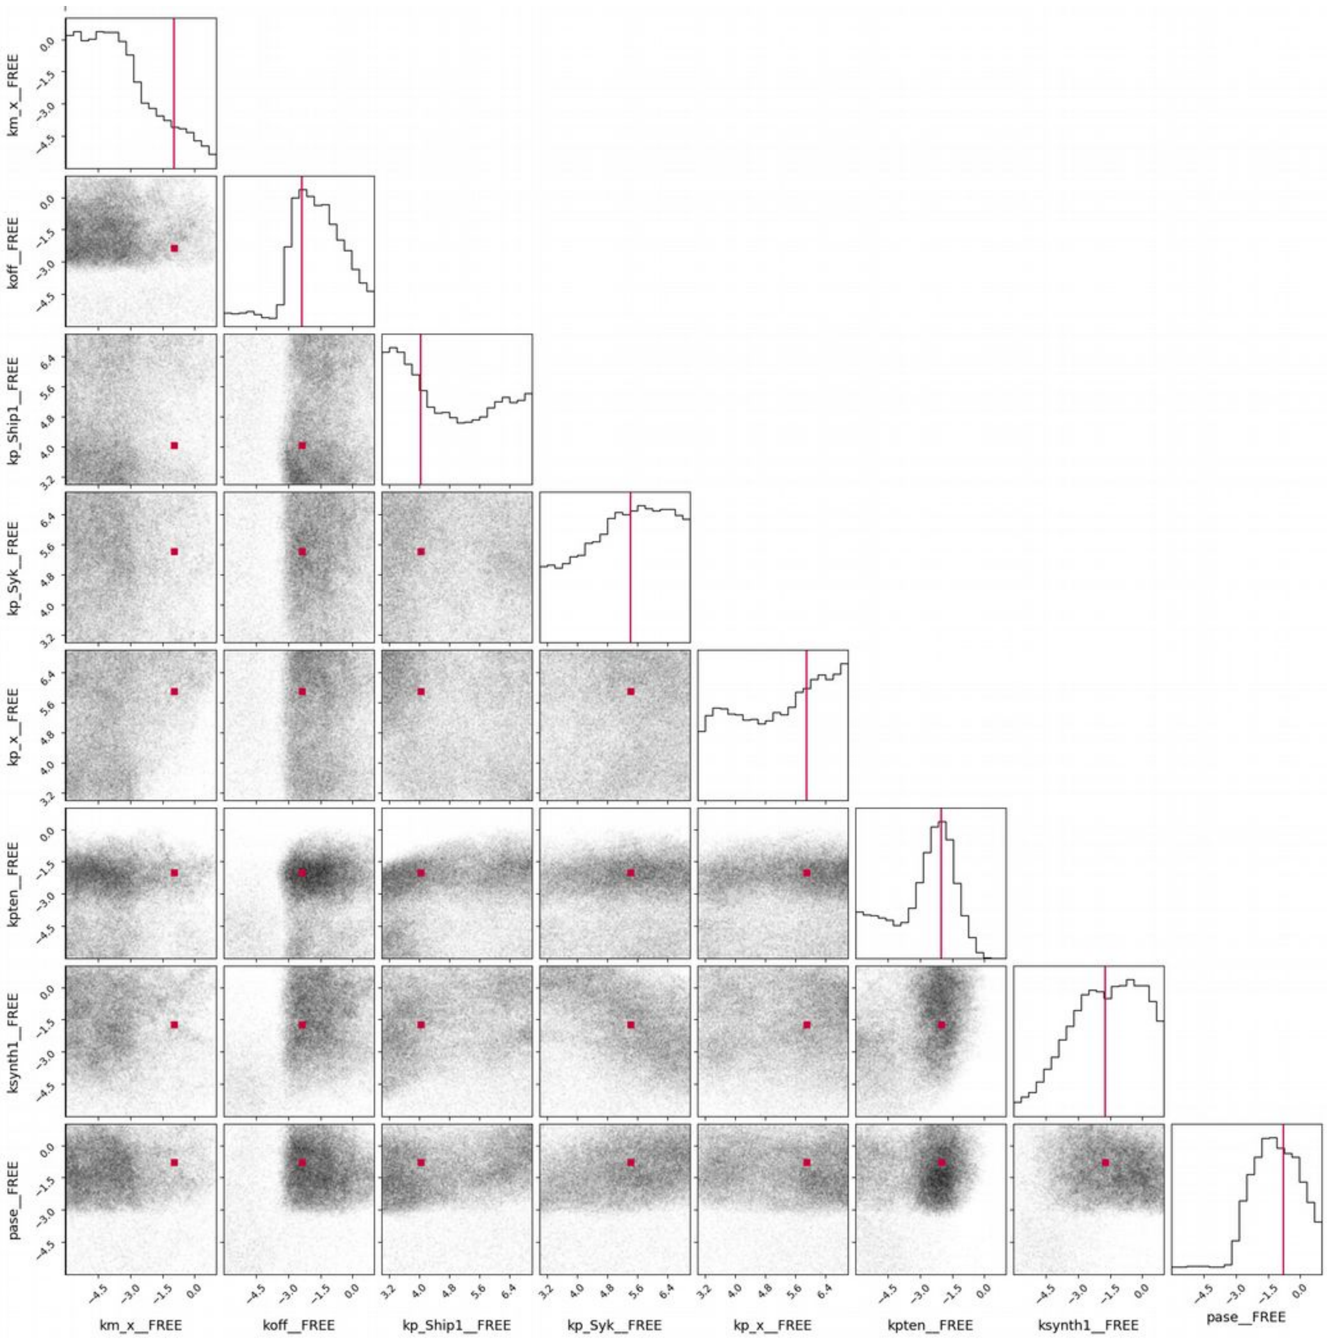
km_x__FREE
koff__FREE
kp_Ship1__FREE
kp_Syk__FREE
kp_x__FREE
kpten__FREE
ksynth1__FREE
pase__FREE

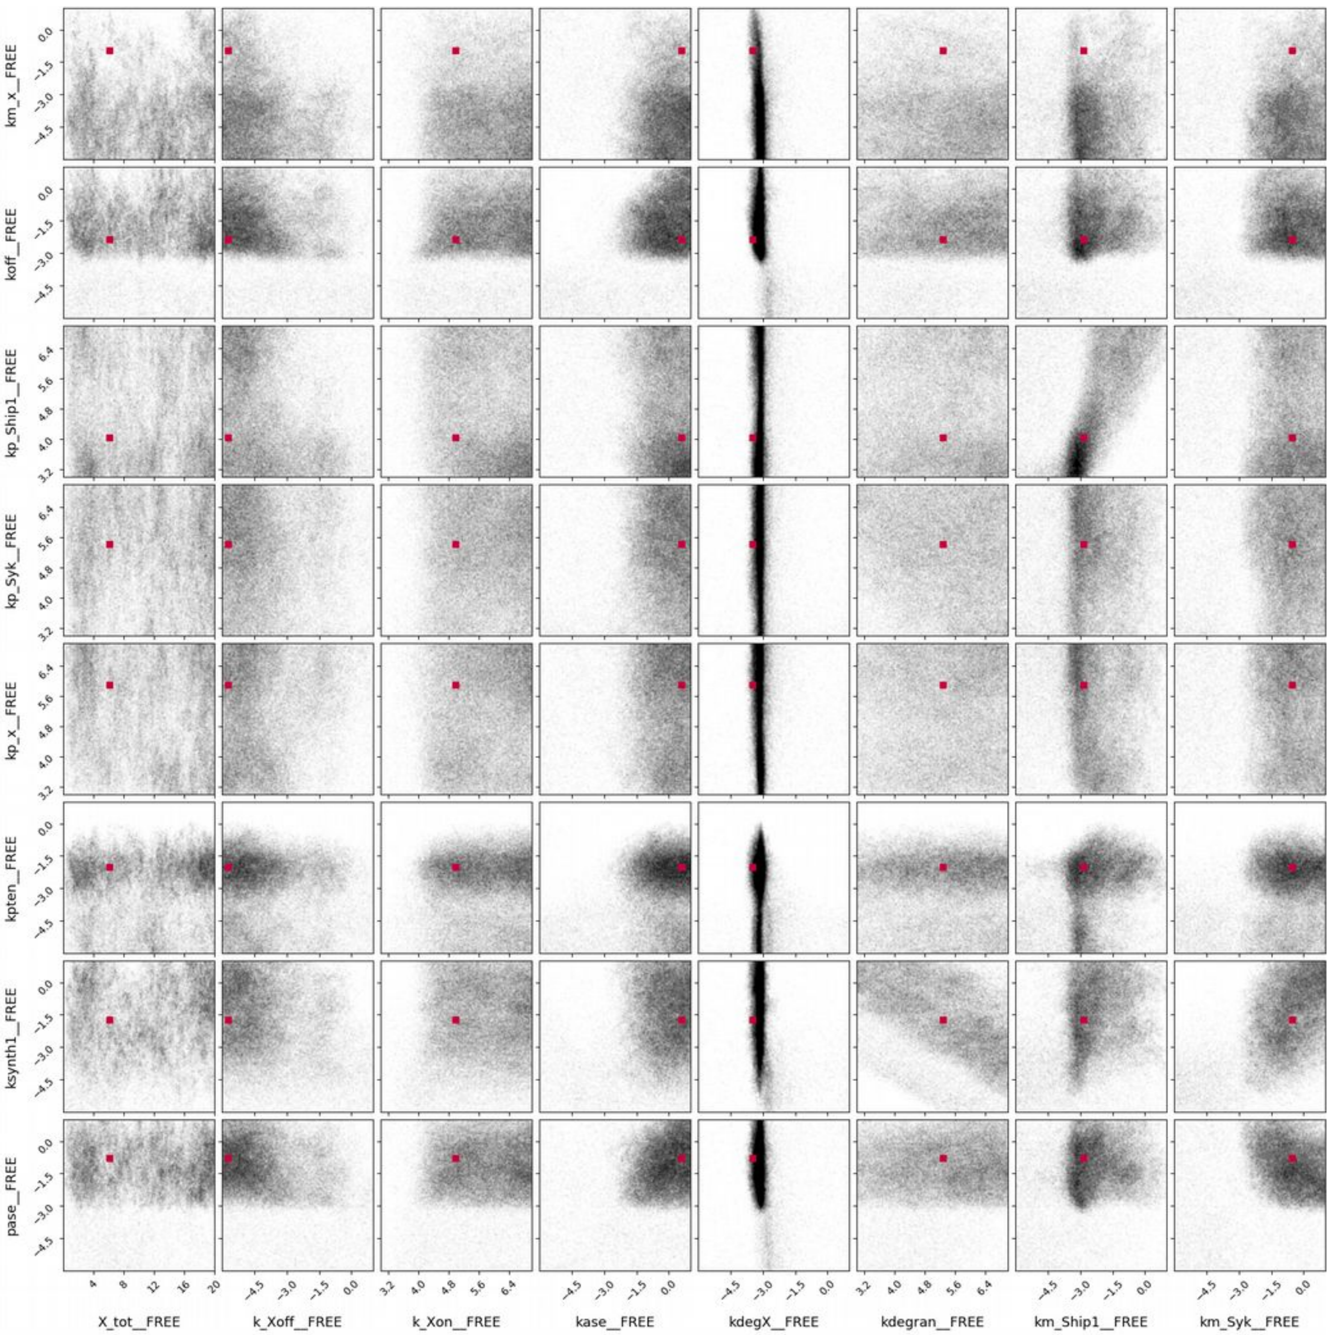


Figure S5: Corner plot showing the marginal posterior distribution for each pair of model parameters, under a measurement protocol consisting of 64 qualitative measurements, each with two possible categorical outcomes. The plot is split over the previous three pages for display purposes. Ground truth parameters are shown in red.

4 three-category qualitative measurements

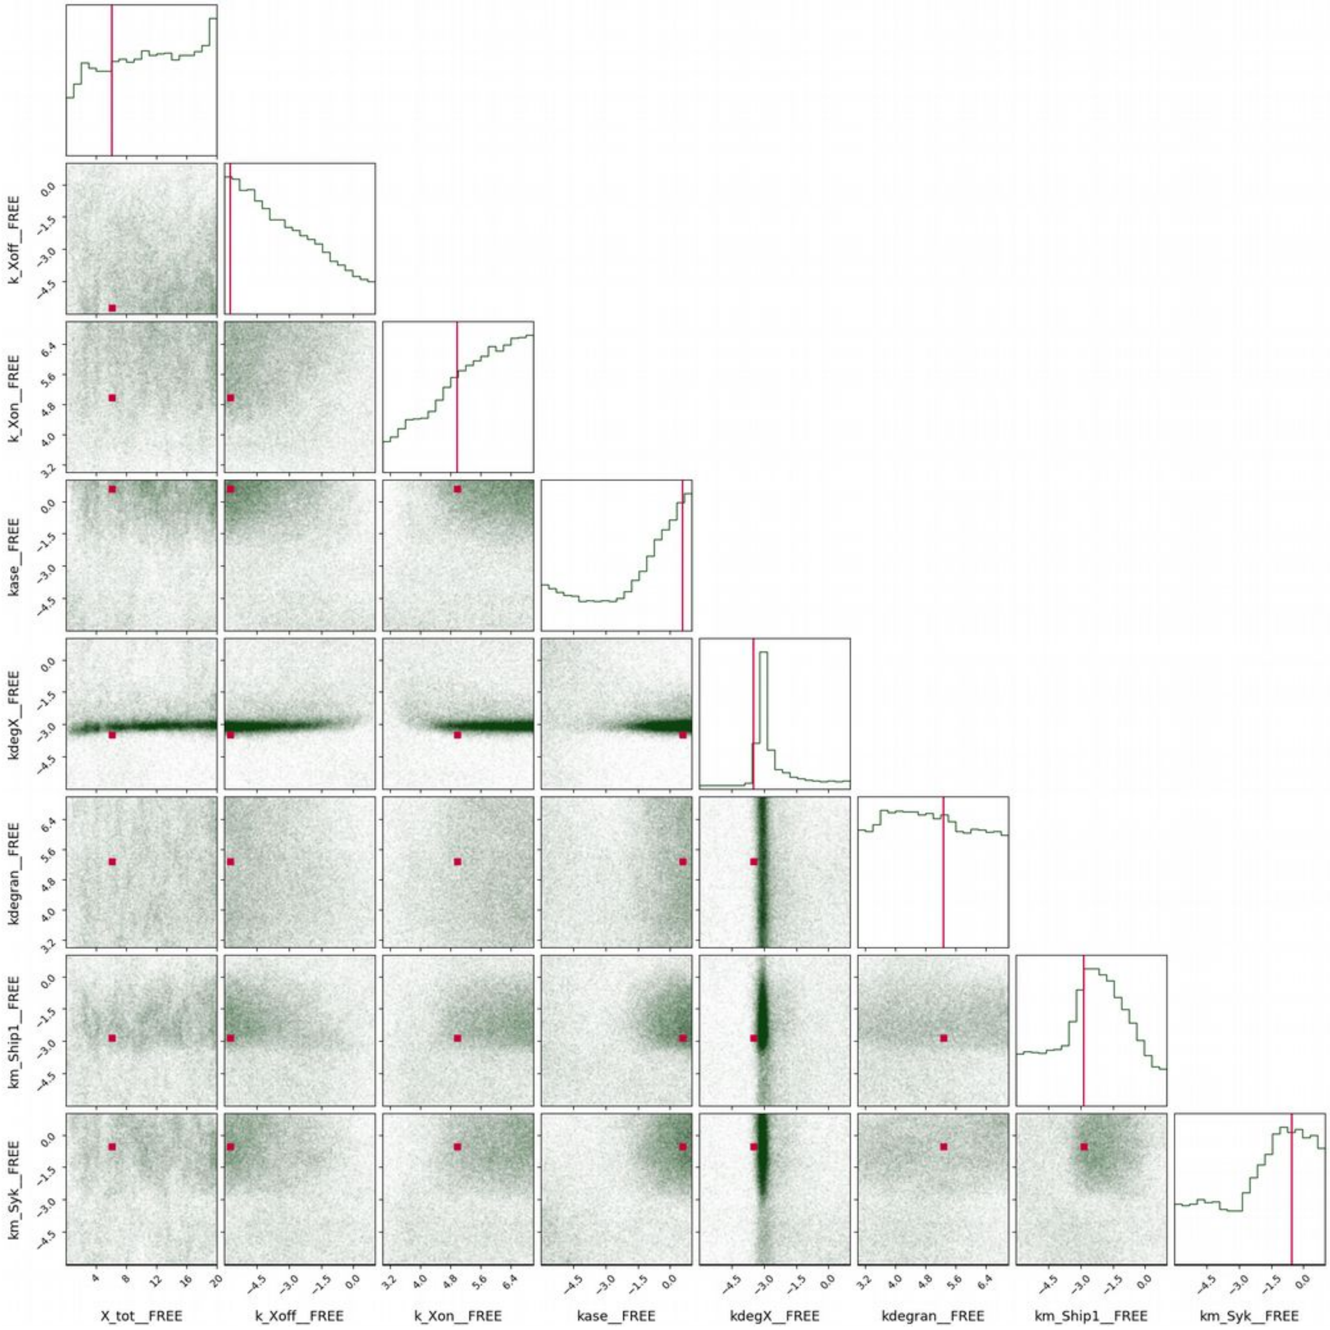

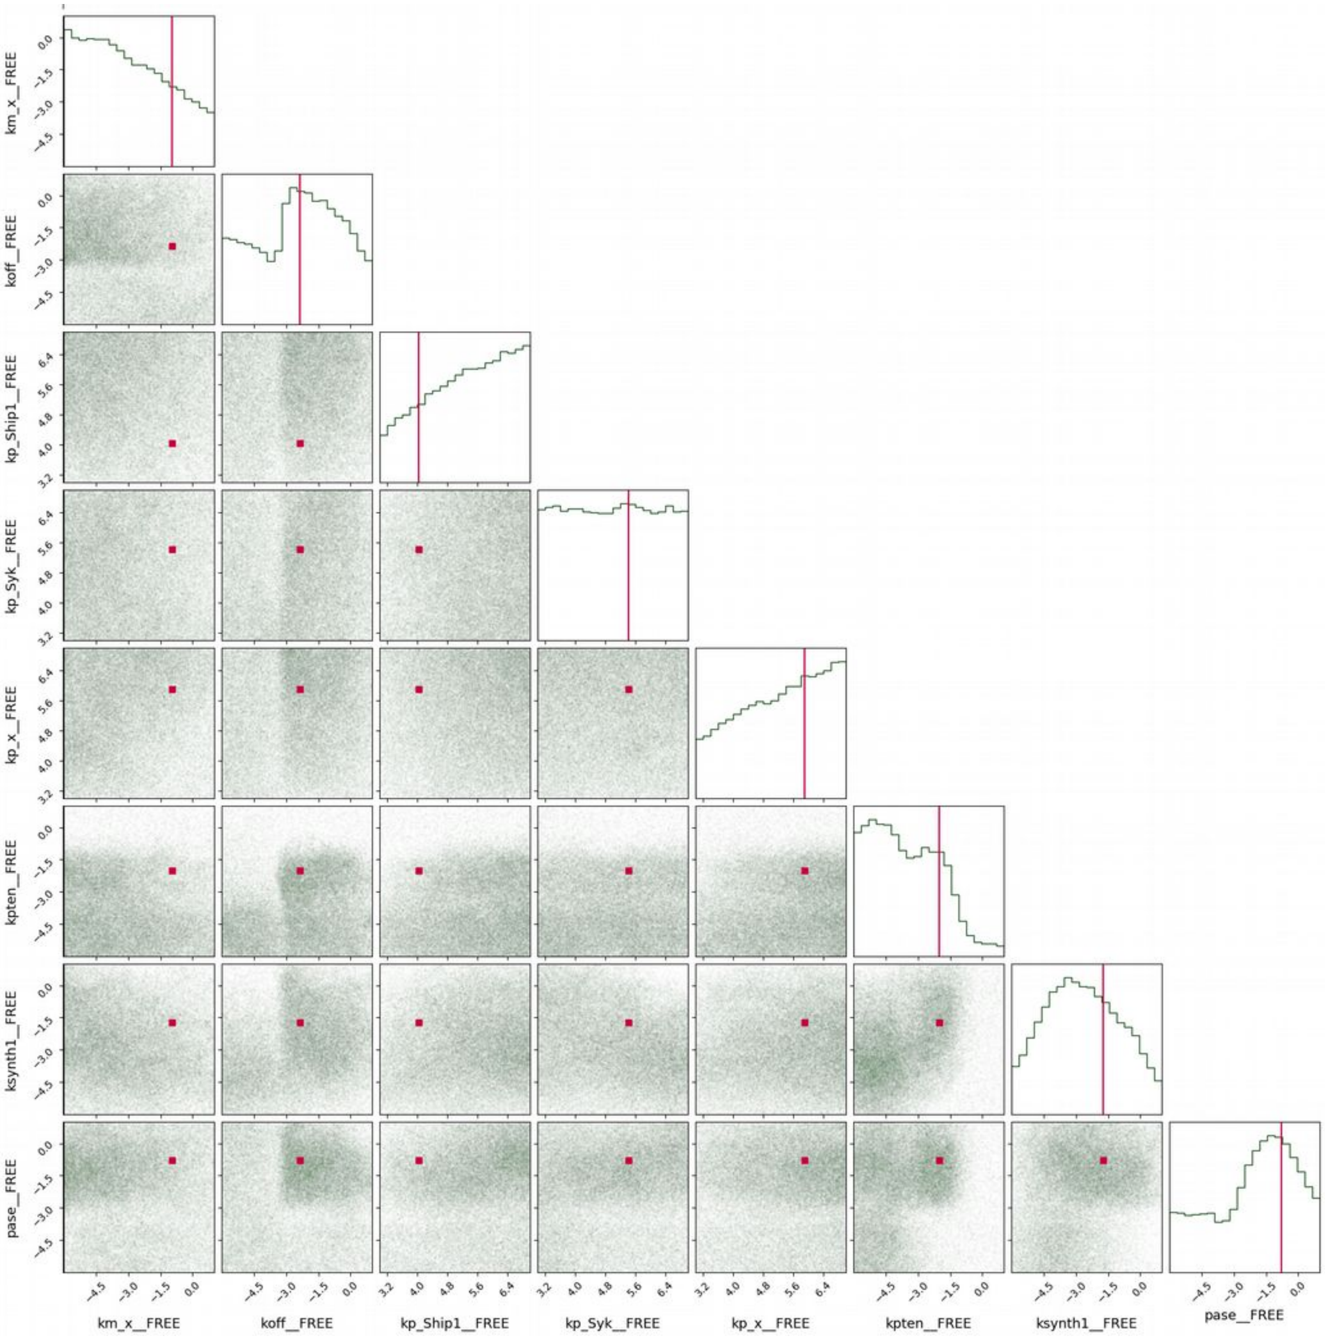
km_x__FREE
koff__FREE
kp_Ship1__FREE
kp_Syk__FREE
kp_x__FREE
kpten__FREE
ksynth1__FREE
pase__FREE

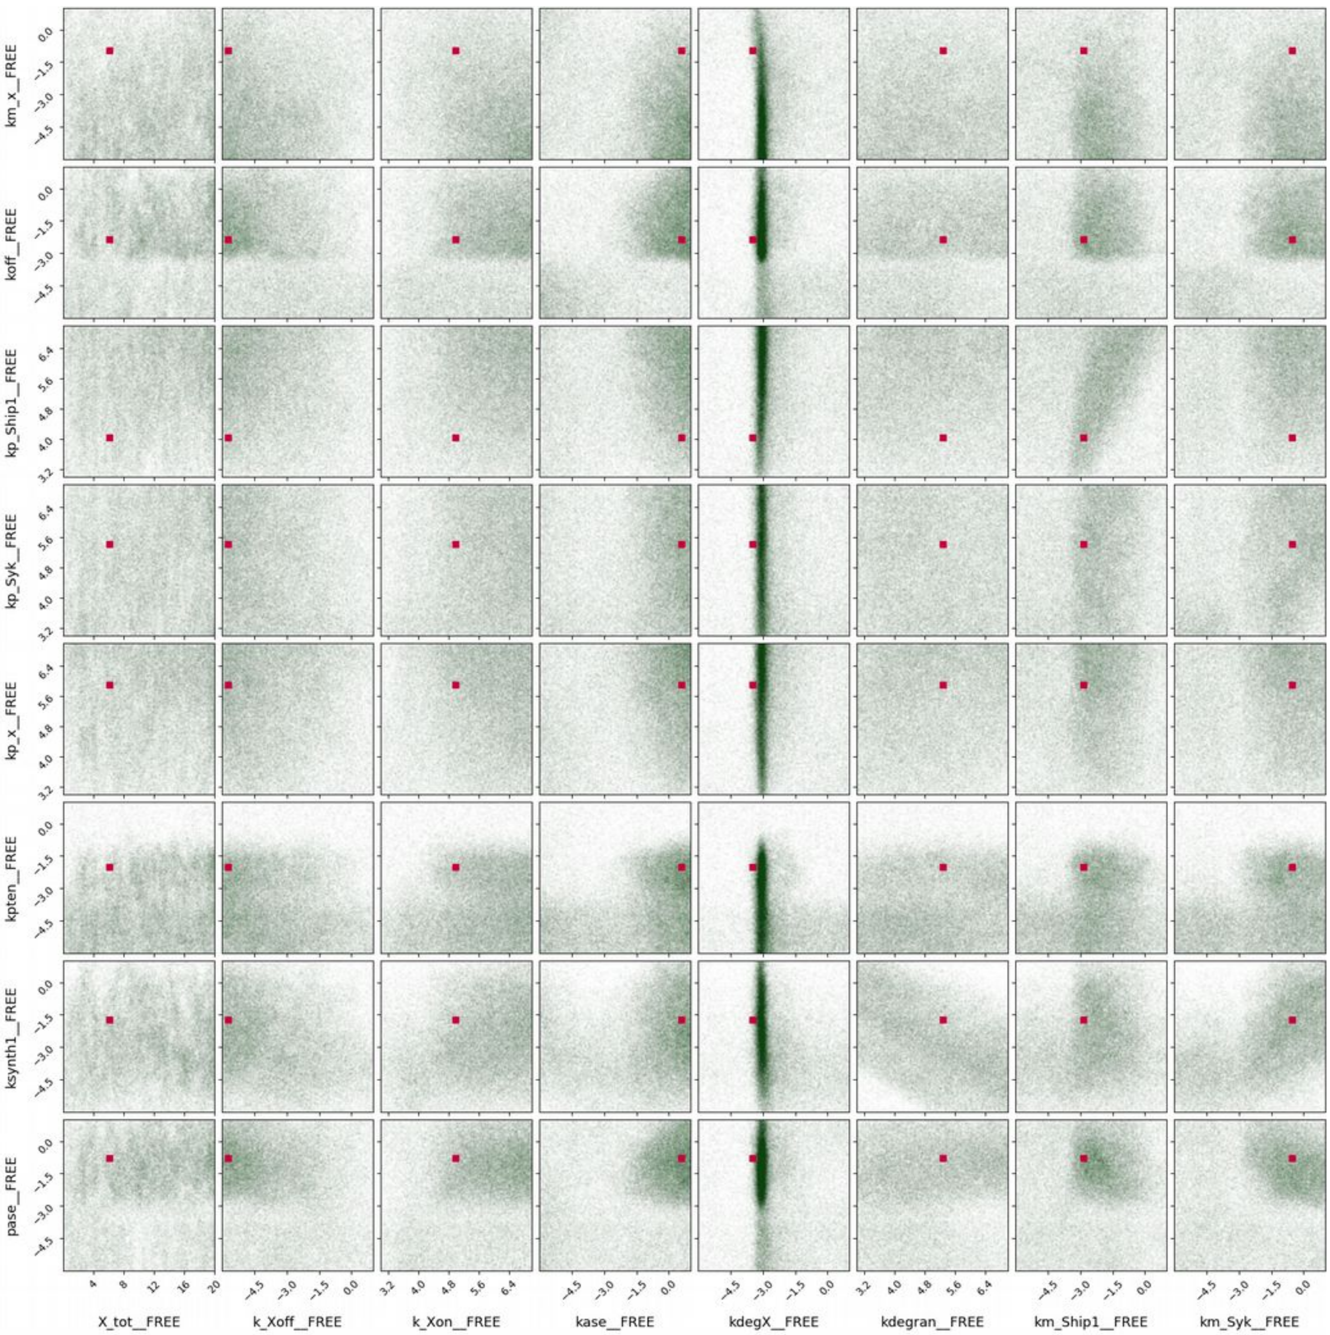


Figure S6: Corner plot showing the marginal posterior distribution for each pair of model parameters, under a measurement protocol consisting of 4 qualitative measurements, each with three possible categorical outcomes. The plot is split over the previous three pages for display purposes. Ground truth parameters are shown in red.

8 three-category qualitative measurements

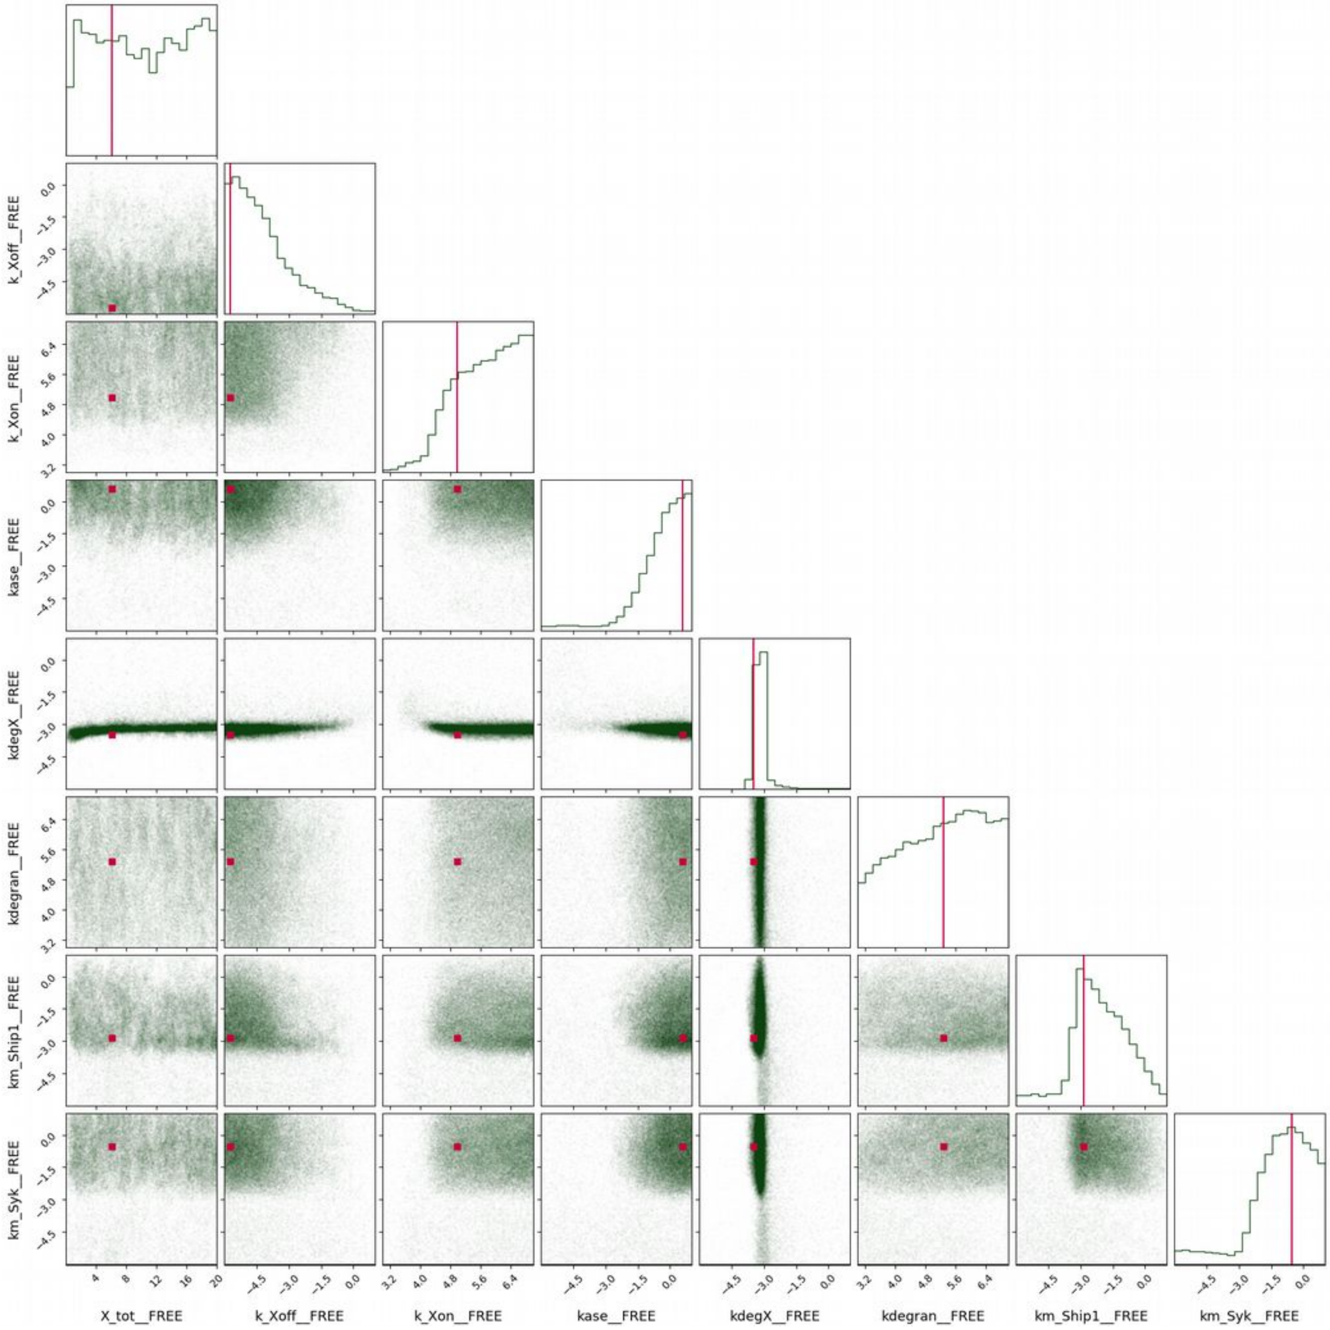

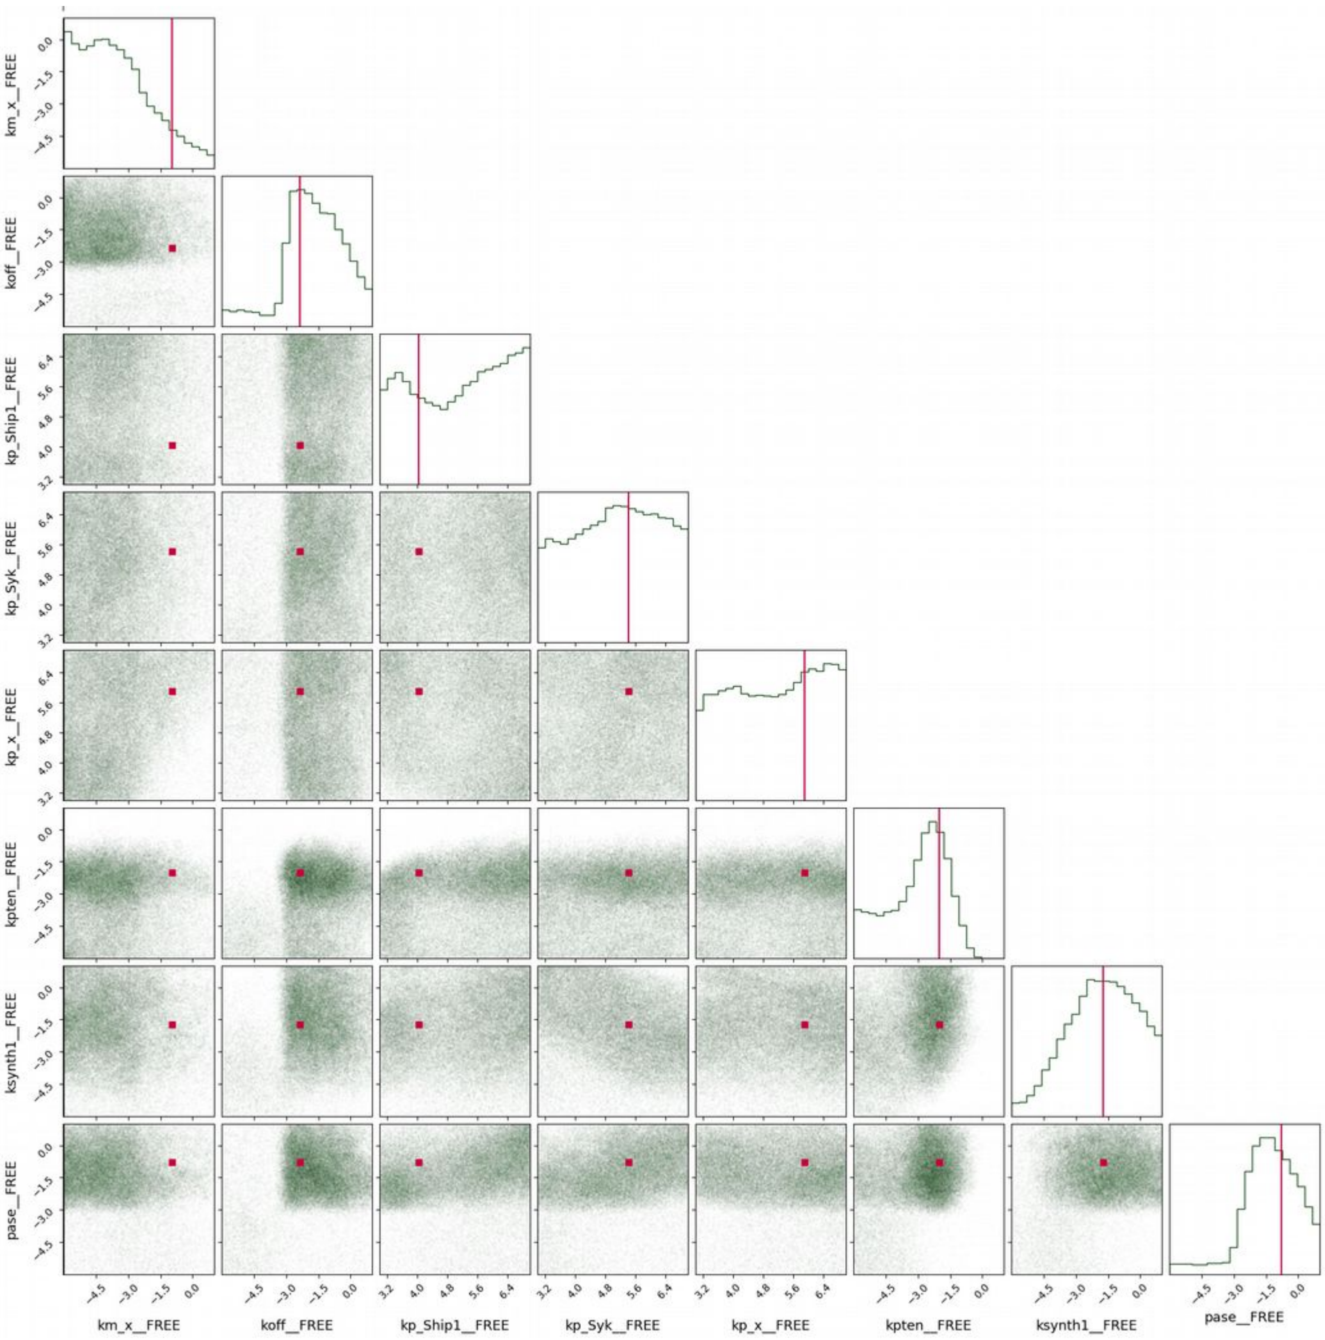
km_x__FREE
koff__FREE
kp_Ship1__FREE
kp_Syk__FREE
kp_x__FREE
kpten__FREE
ksynth1__FREE
pase__FREE

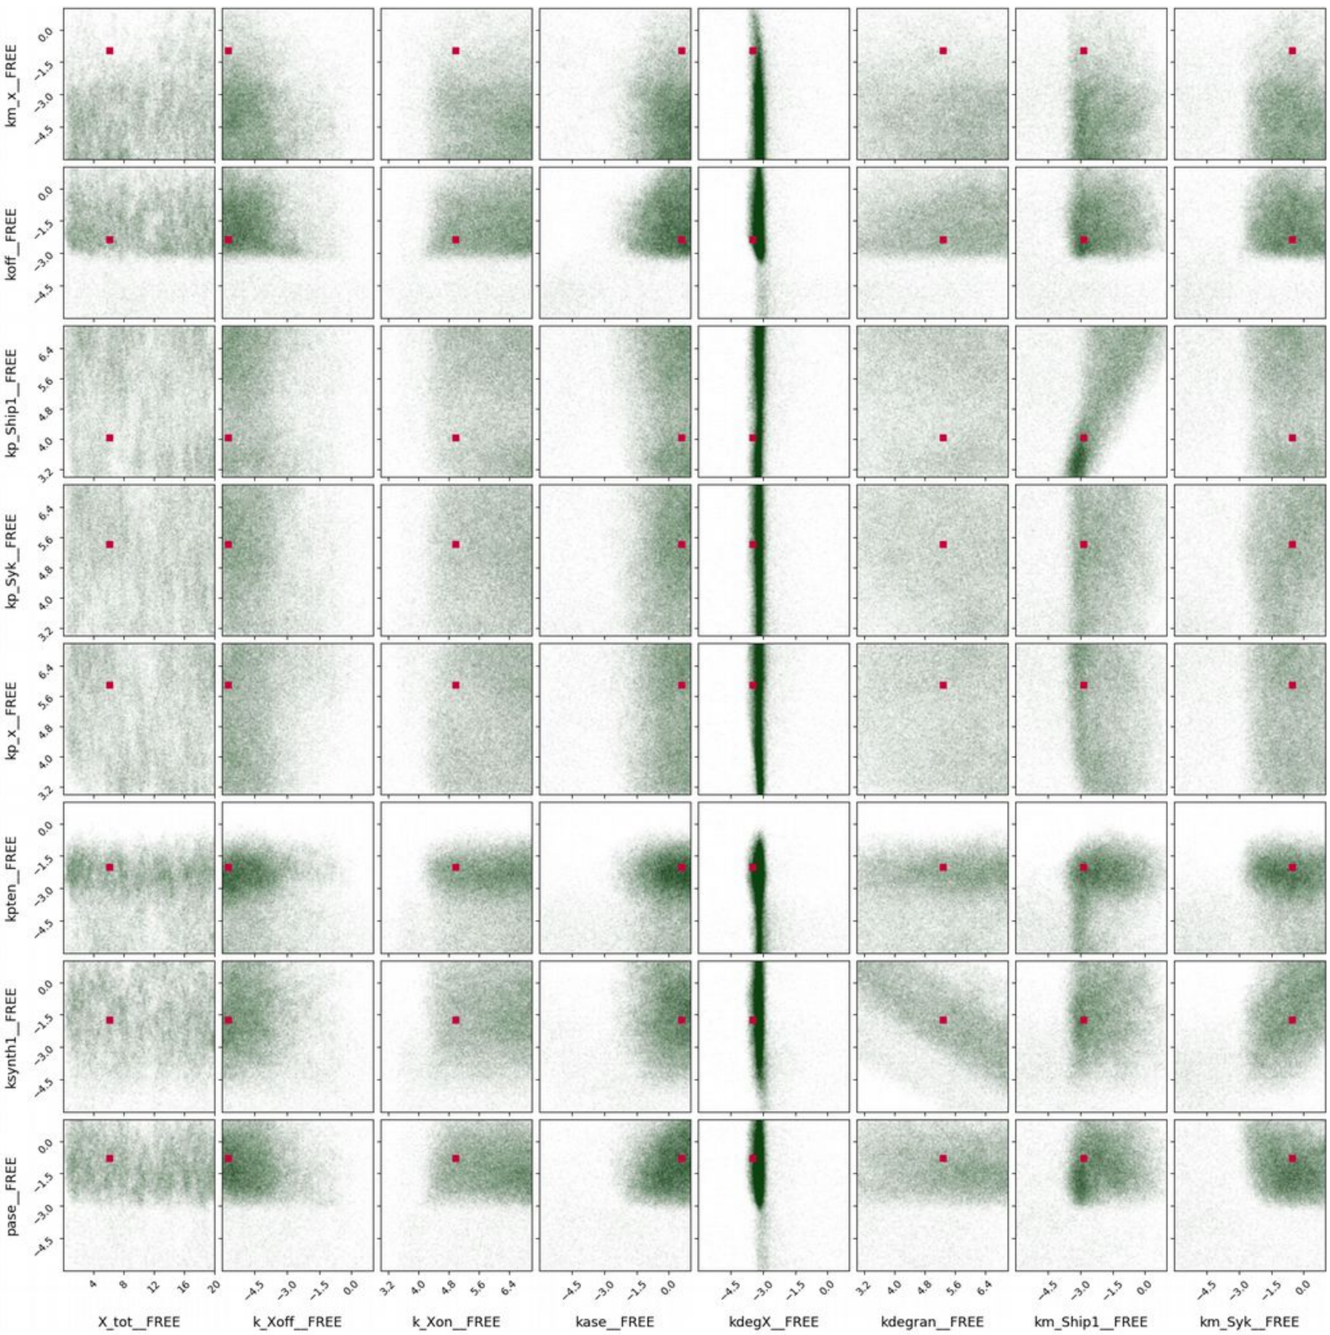


Figure S7: Corner plot showing the marginal posterior distribution for each pair of model parameters, under a measurement protocol consisting of 8 qualitative measurements, each with three possible categorical outcomes. The plot is split over the previous three pages for display purposes. Ground truth parameters are shown in red.

16 three-category qualitative measurements

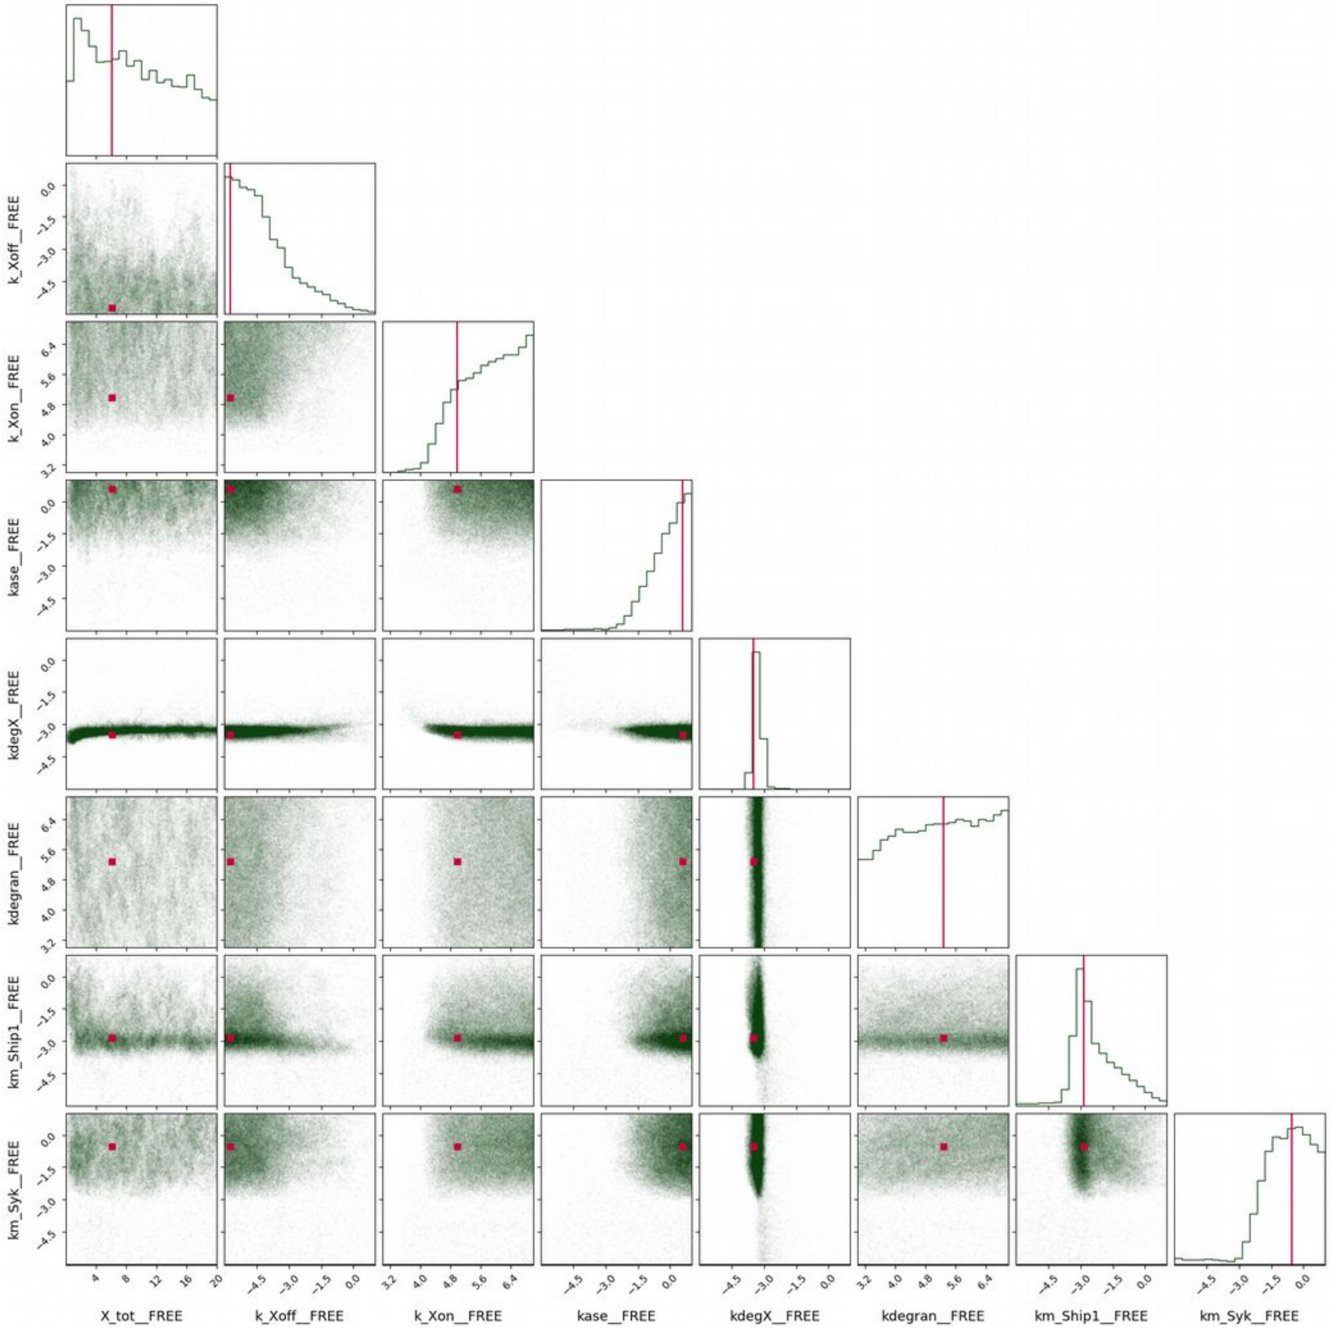

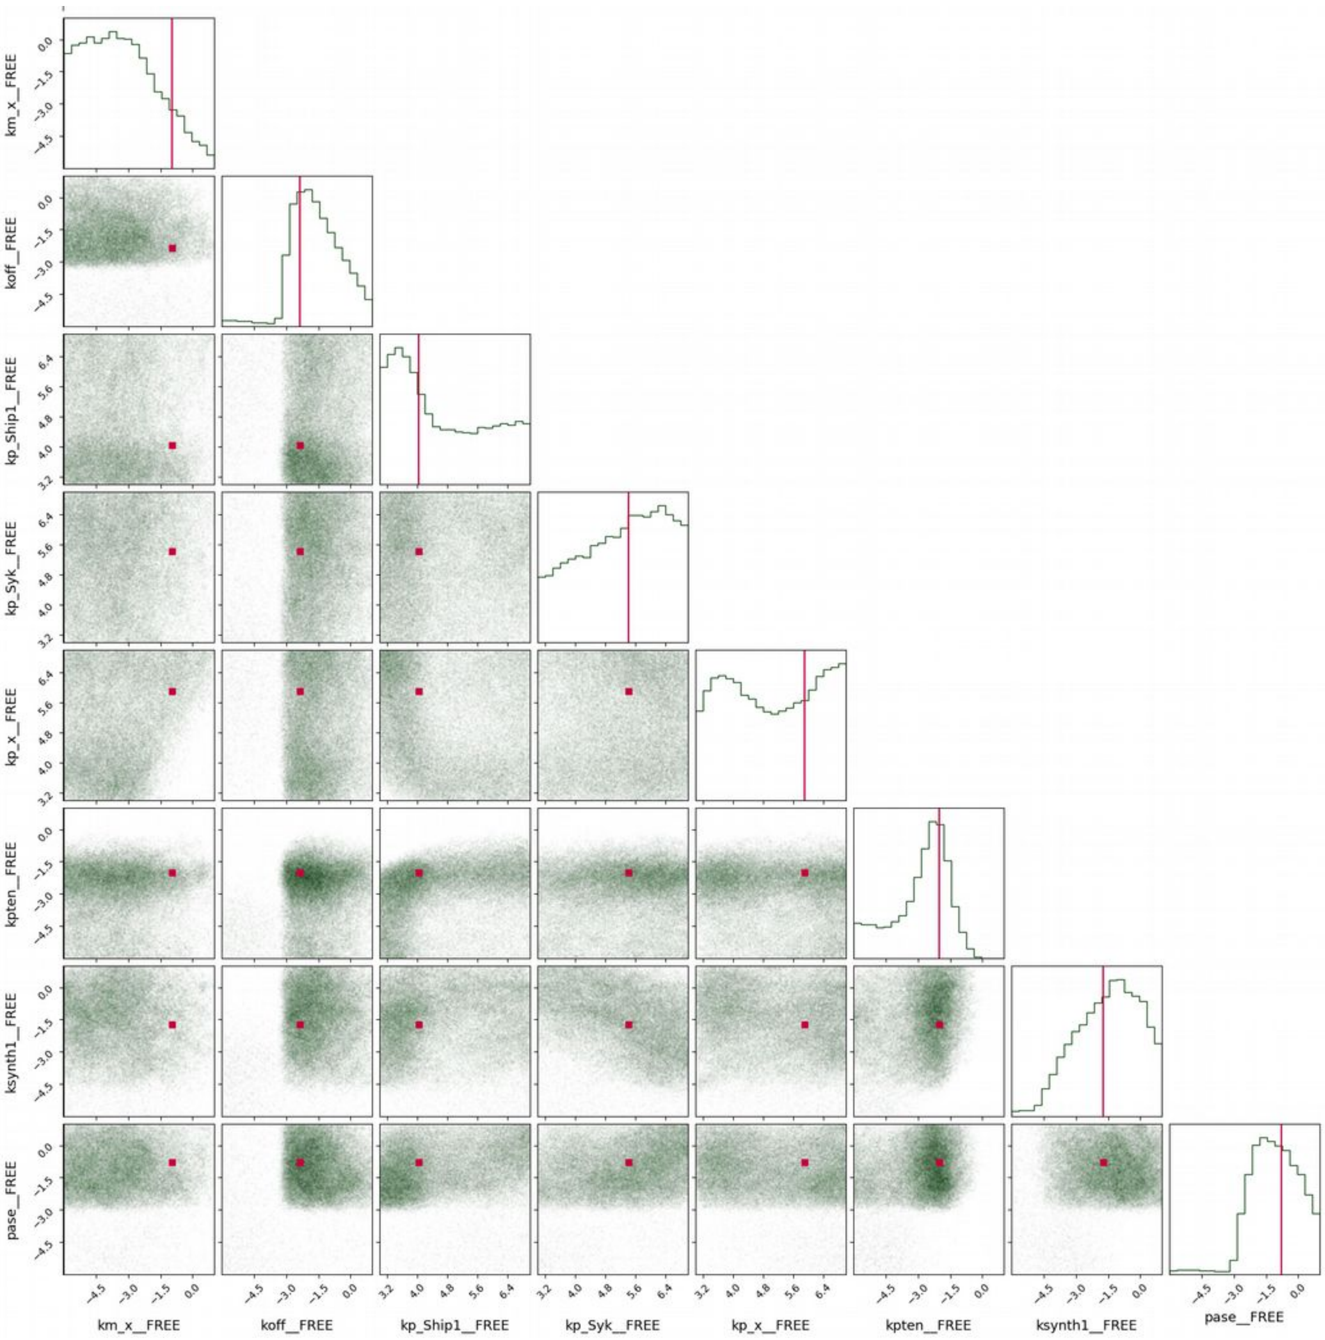

km_x__FREE
koff__FREE
kp_Ship1__FREE
kp_Syk__FREE
kp_x__FREE
kpten__FREE
ksynth1__FREE
pase__FREE

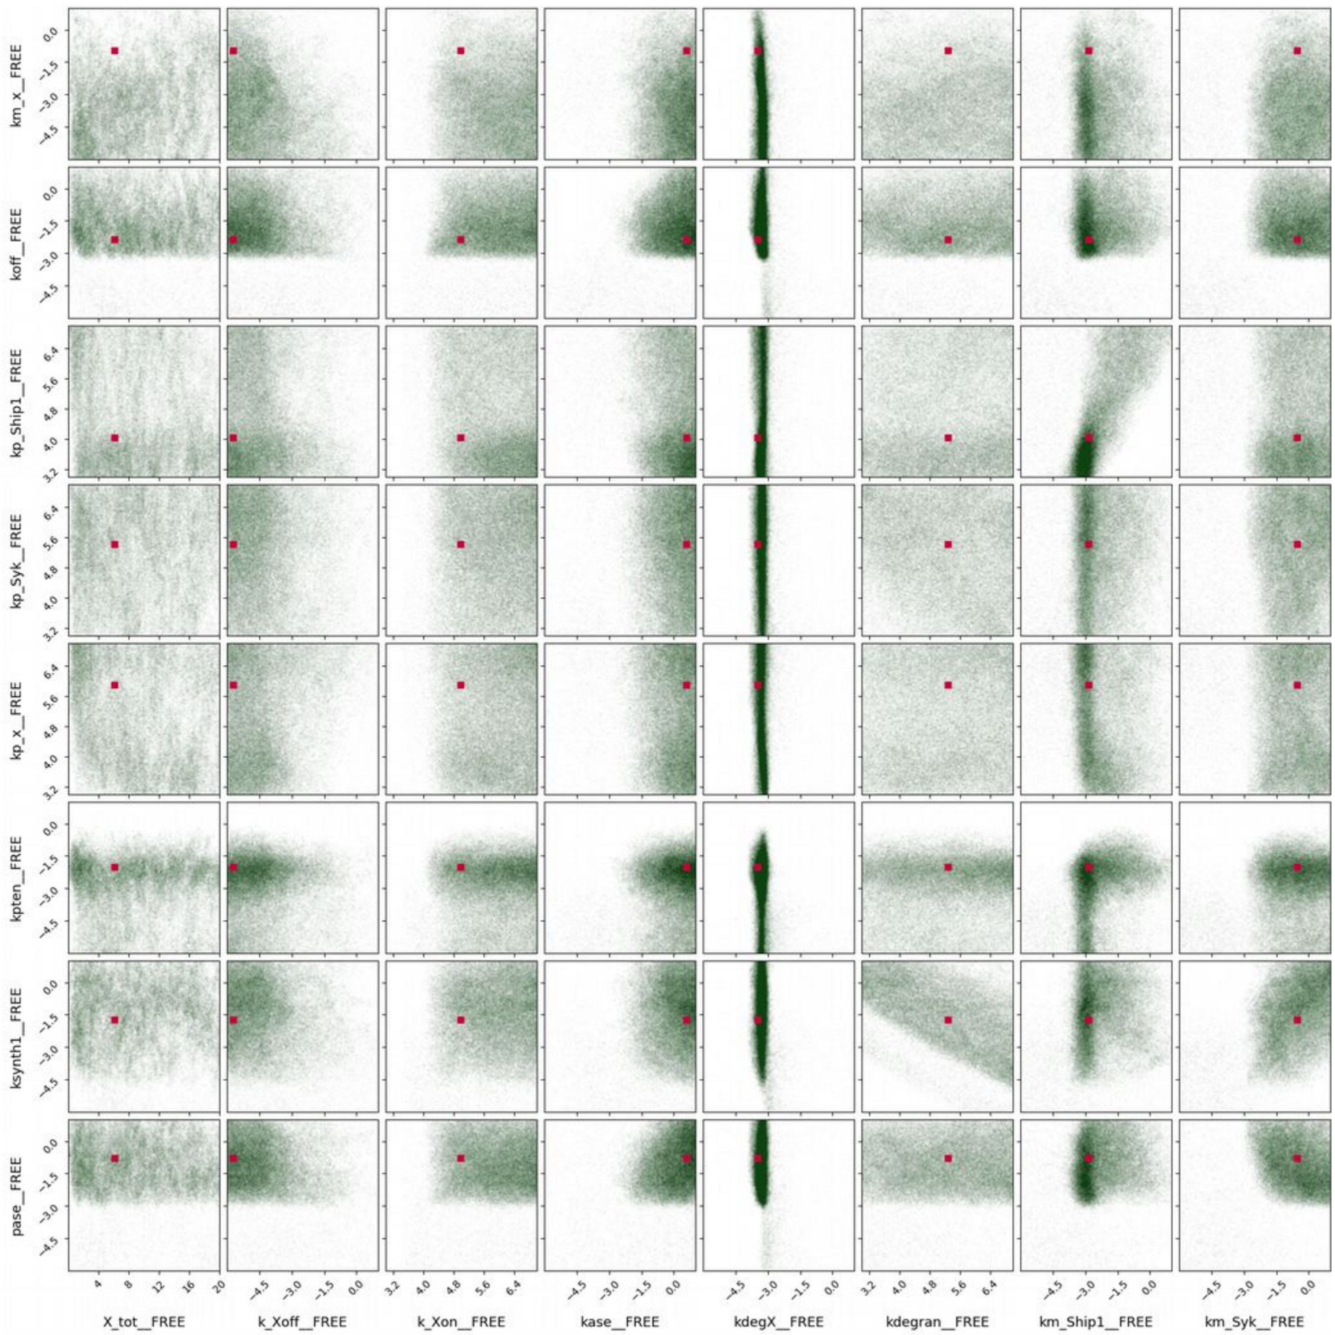


Figure S8: Corner plot showing the marginal posterior distribution for each pair of model parameters, under a measurement protocol consisting of 16 qualitative measurements, each with three possible categorical outcomes. The plot is split over the previous three pages for display purposes. Ground truth parameters are shown in red.

32 three-category qualitative measurements

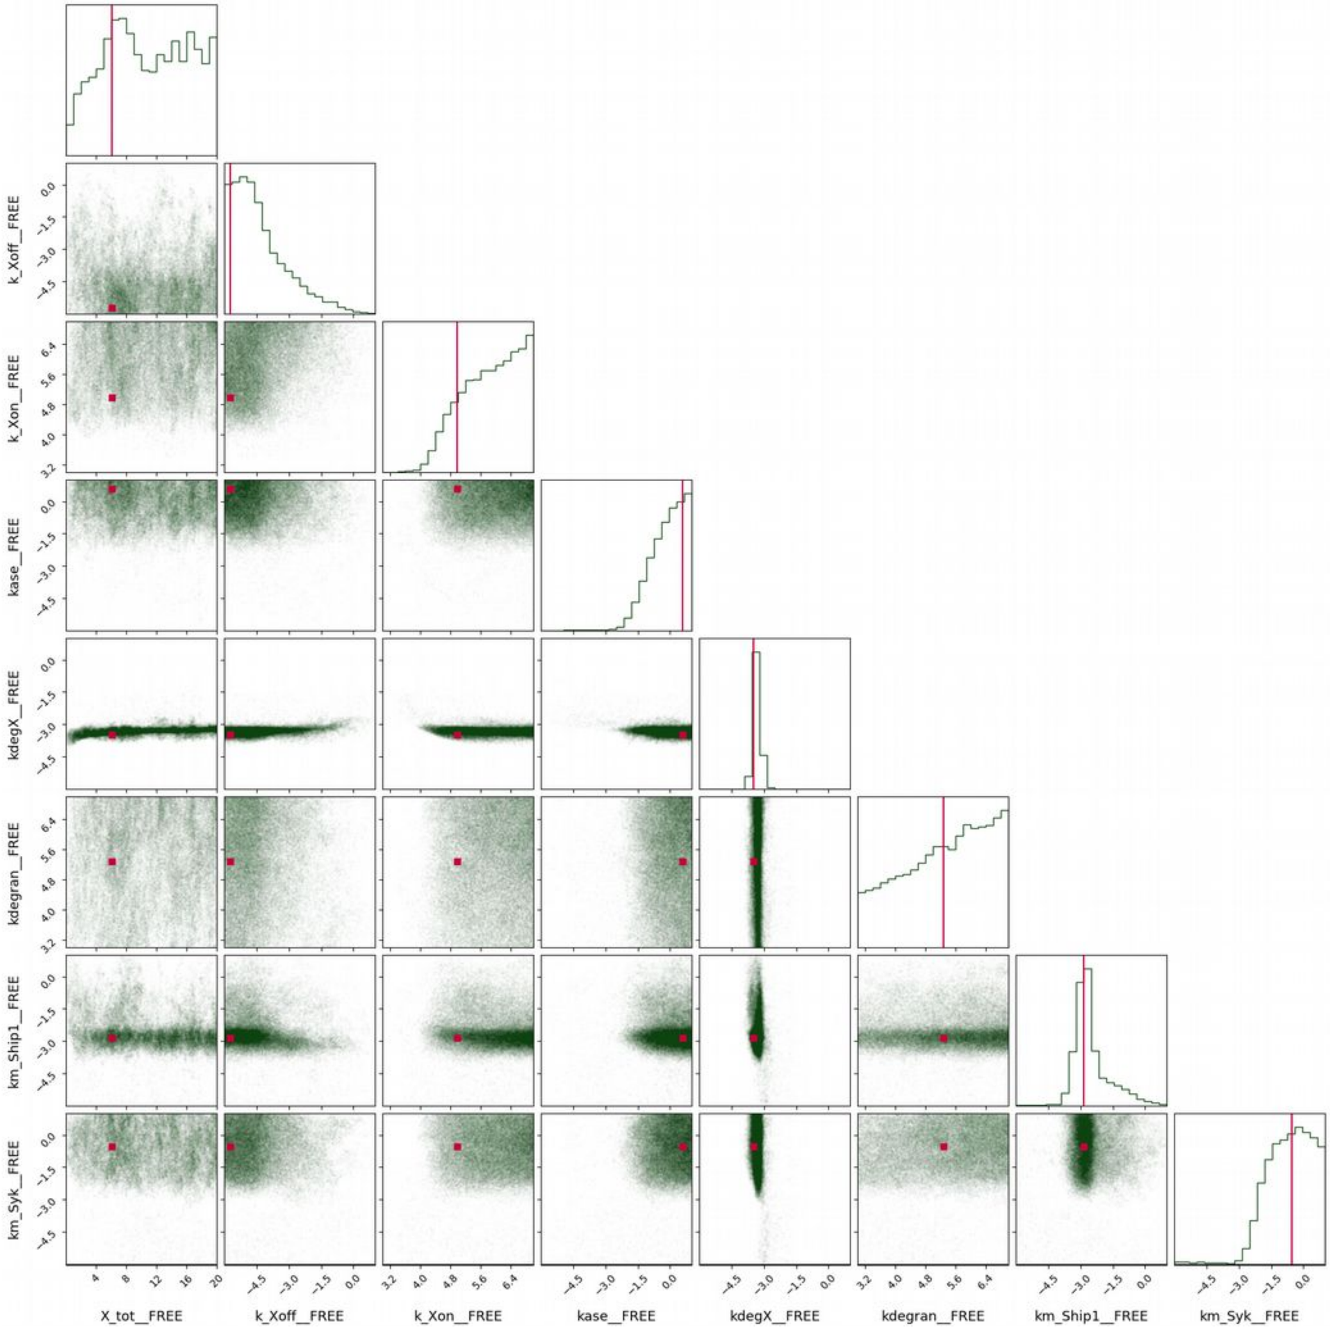

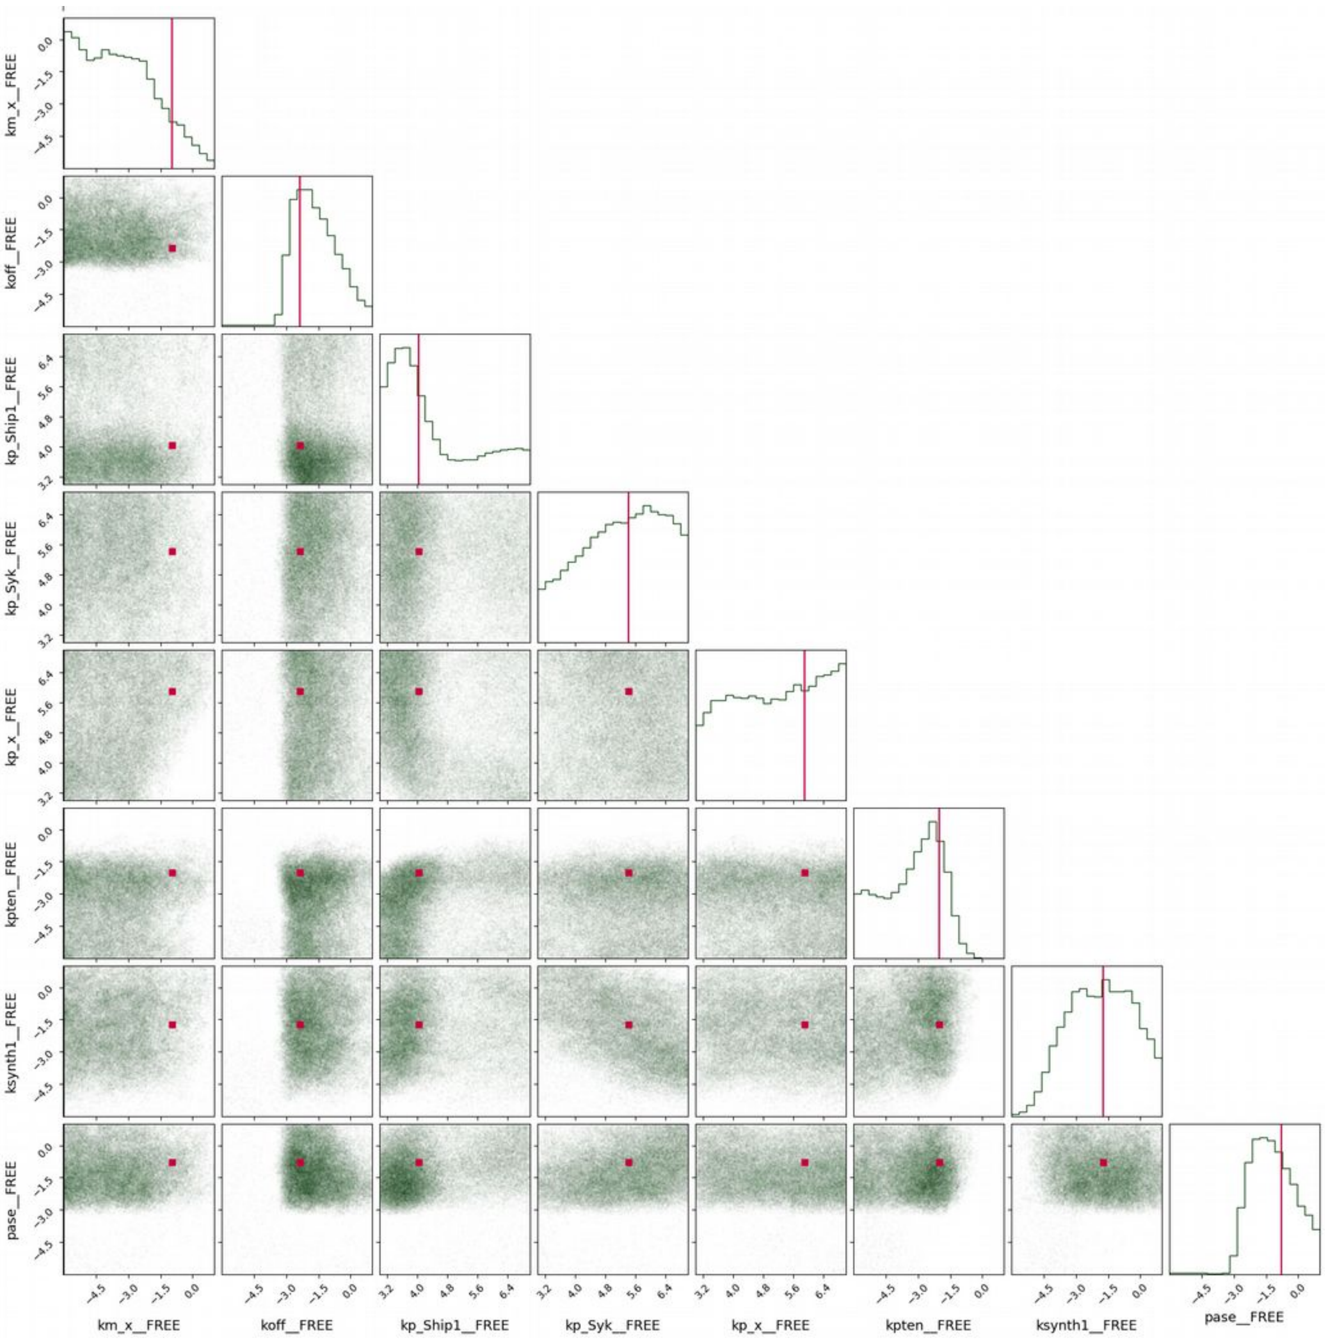
km_x__FREE
koff__FREE
kp_Ship1__FREE
kp_Syk__FREE
kp_x__FREE
kpten__FREE
ksynth1__FREE
pase__FREE

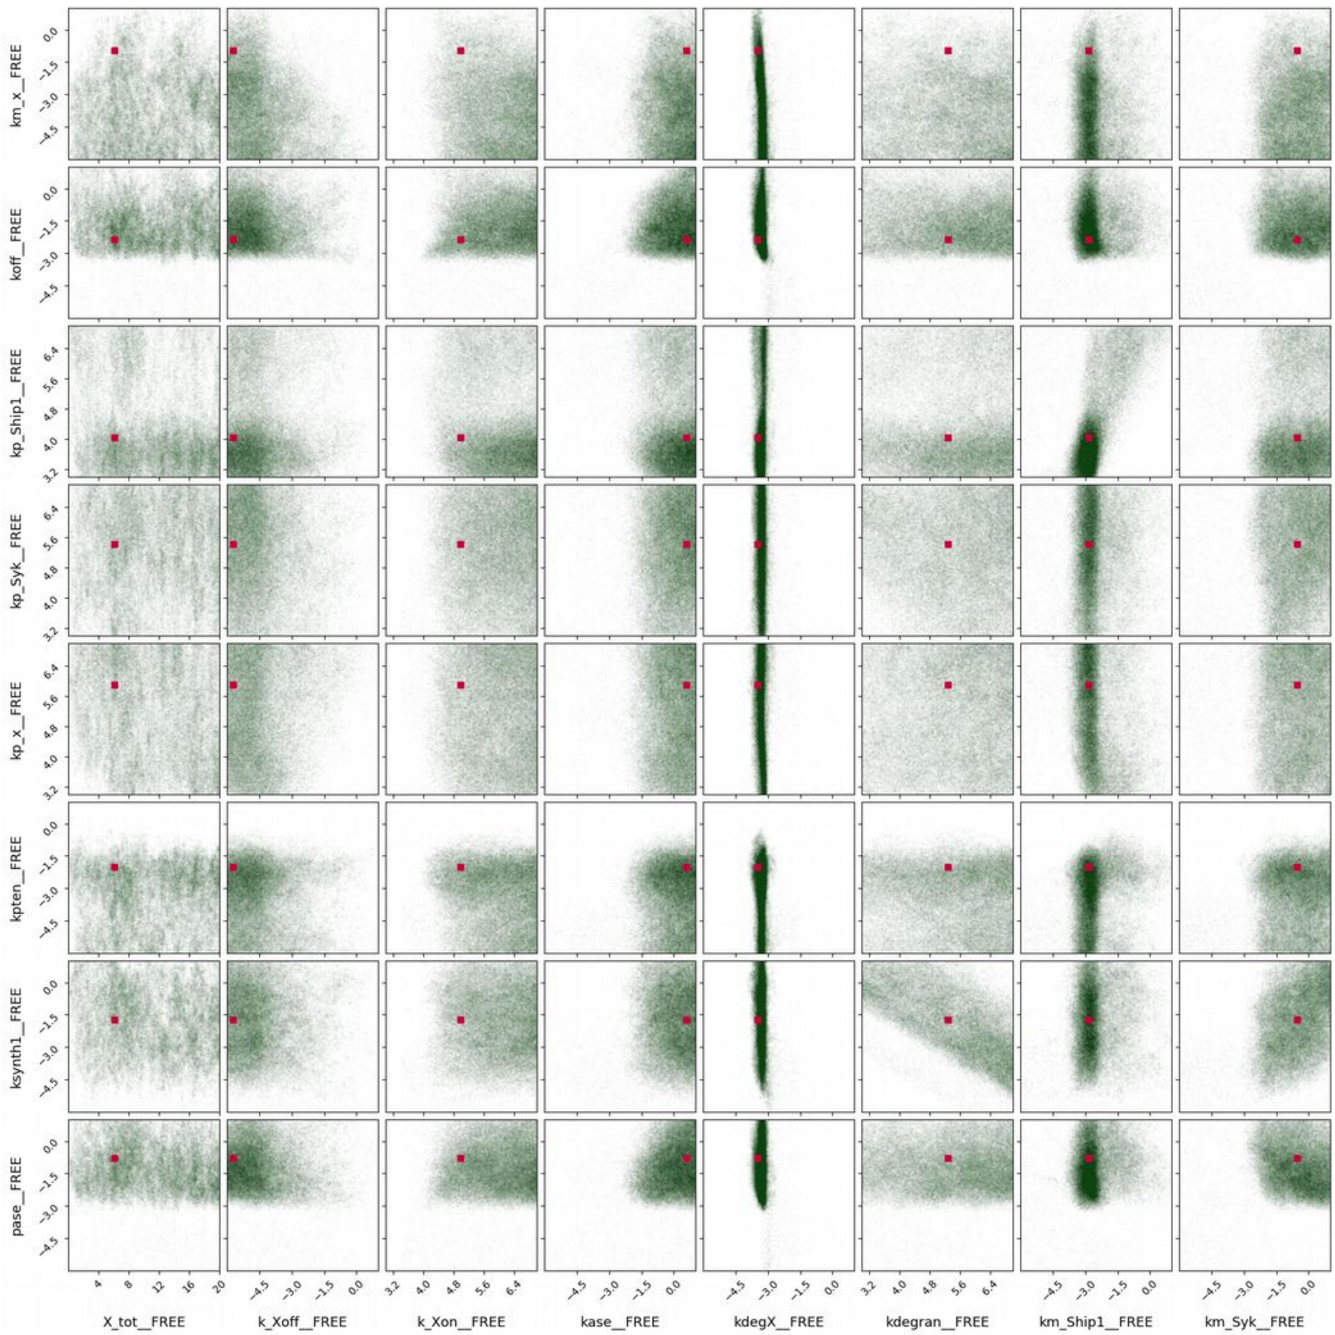


Figure S9: Corner plot showing the marginal posterior distribution for each pair of model parameters, under a measurement protocol consisting of 32 qualitative measurements, each with three possible categorical outcomes. The plot is split over the previous three pages for display purposes. Ground truth parameters are shown in red.

64 three-category measurements

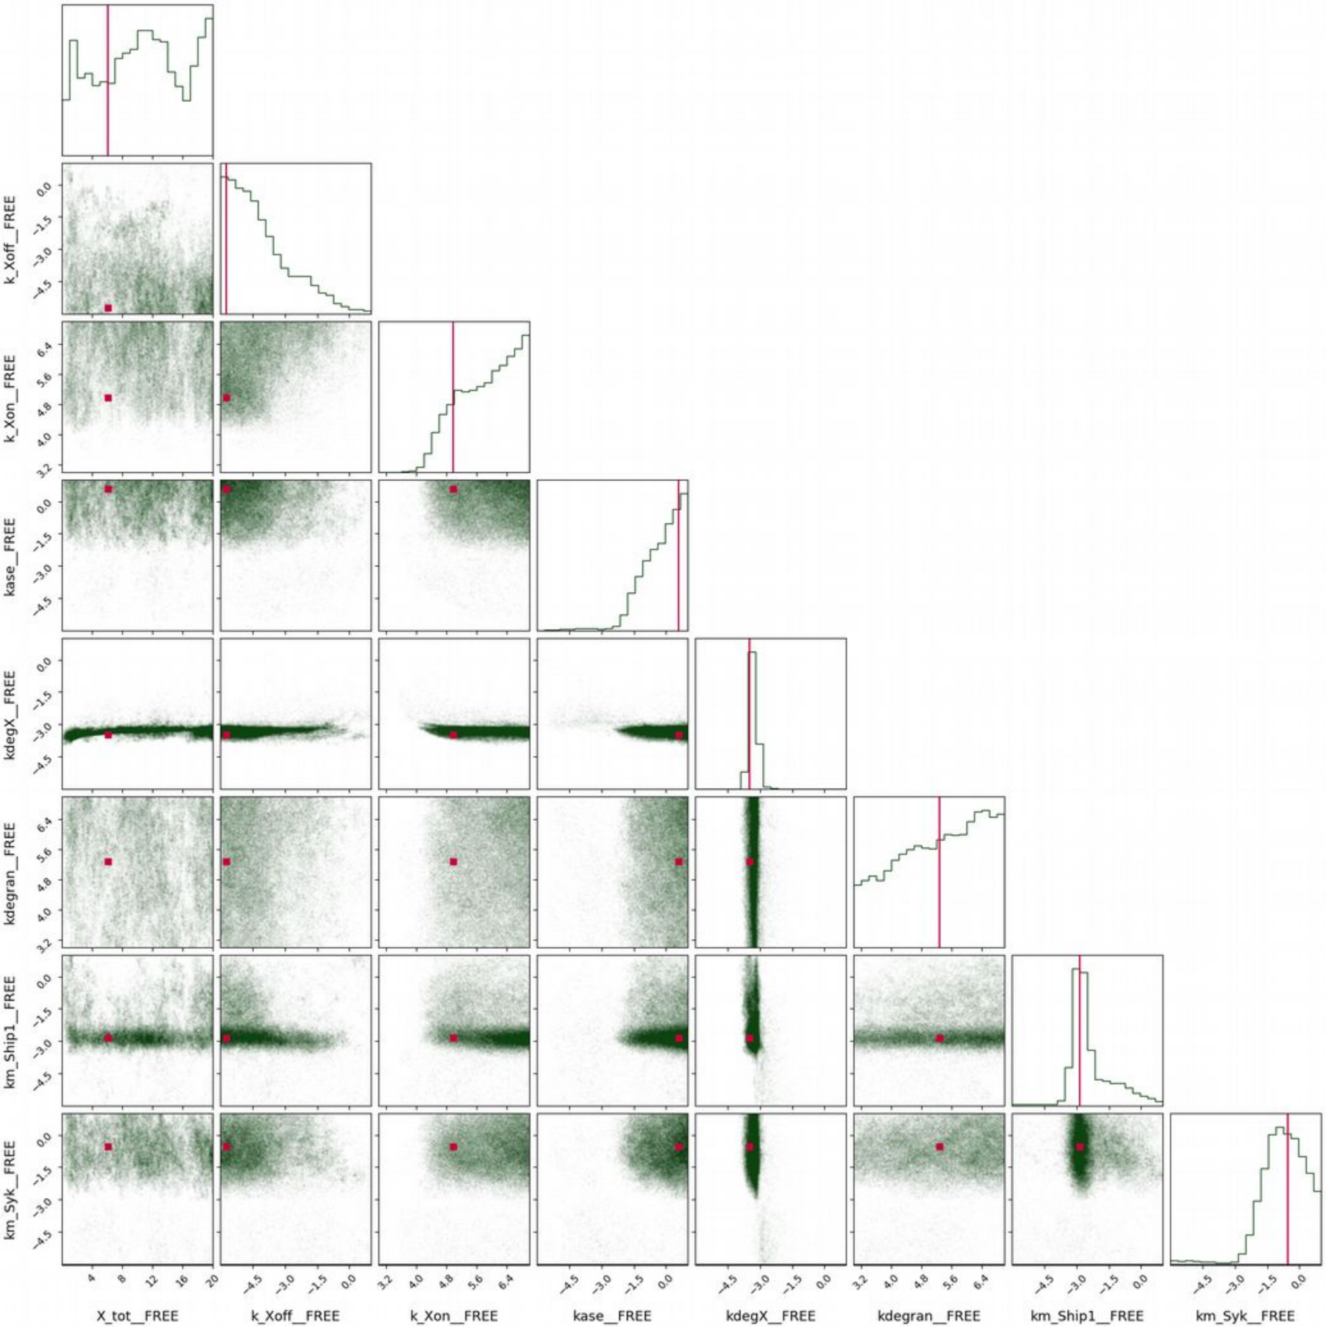

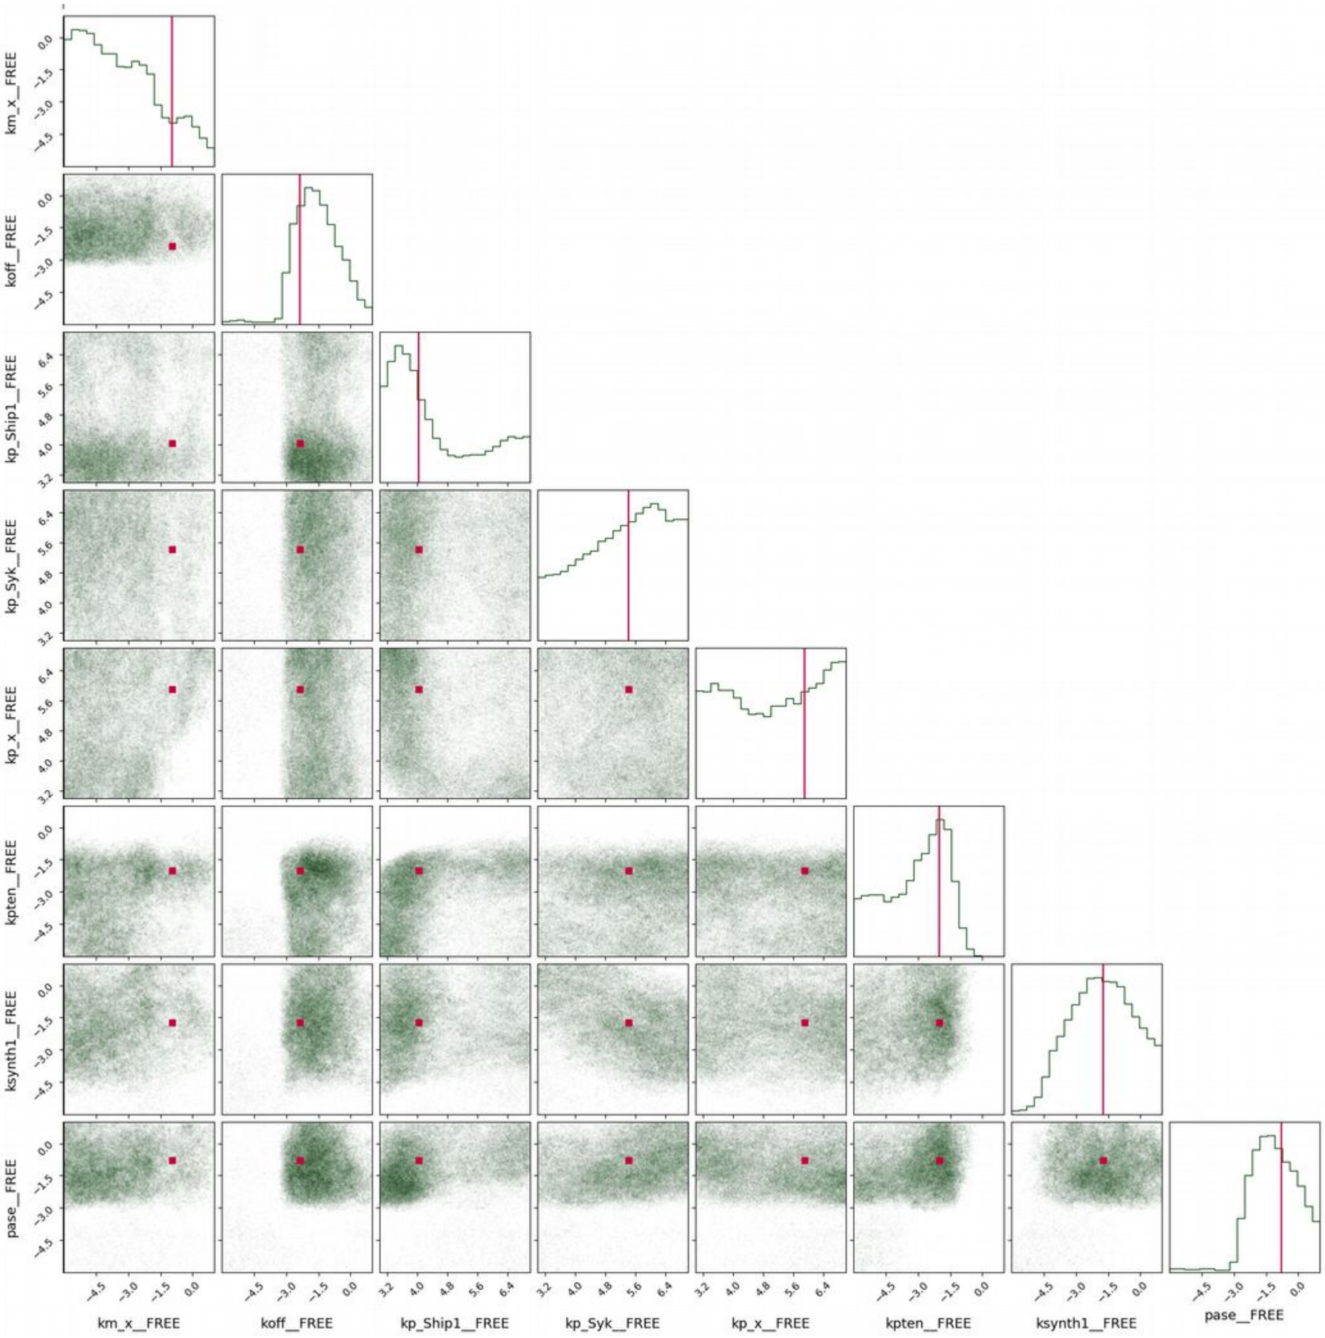

km_x__FREE
koff__FREE
kp_Ship1__FREE
kp_Syk__FREE
kp_x__FREE
kpten__FREE
ksynth1__FREE
pase__FREE

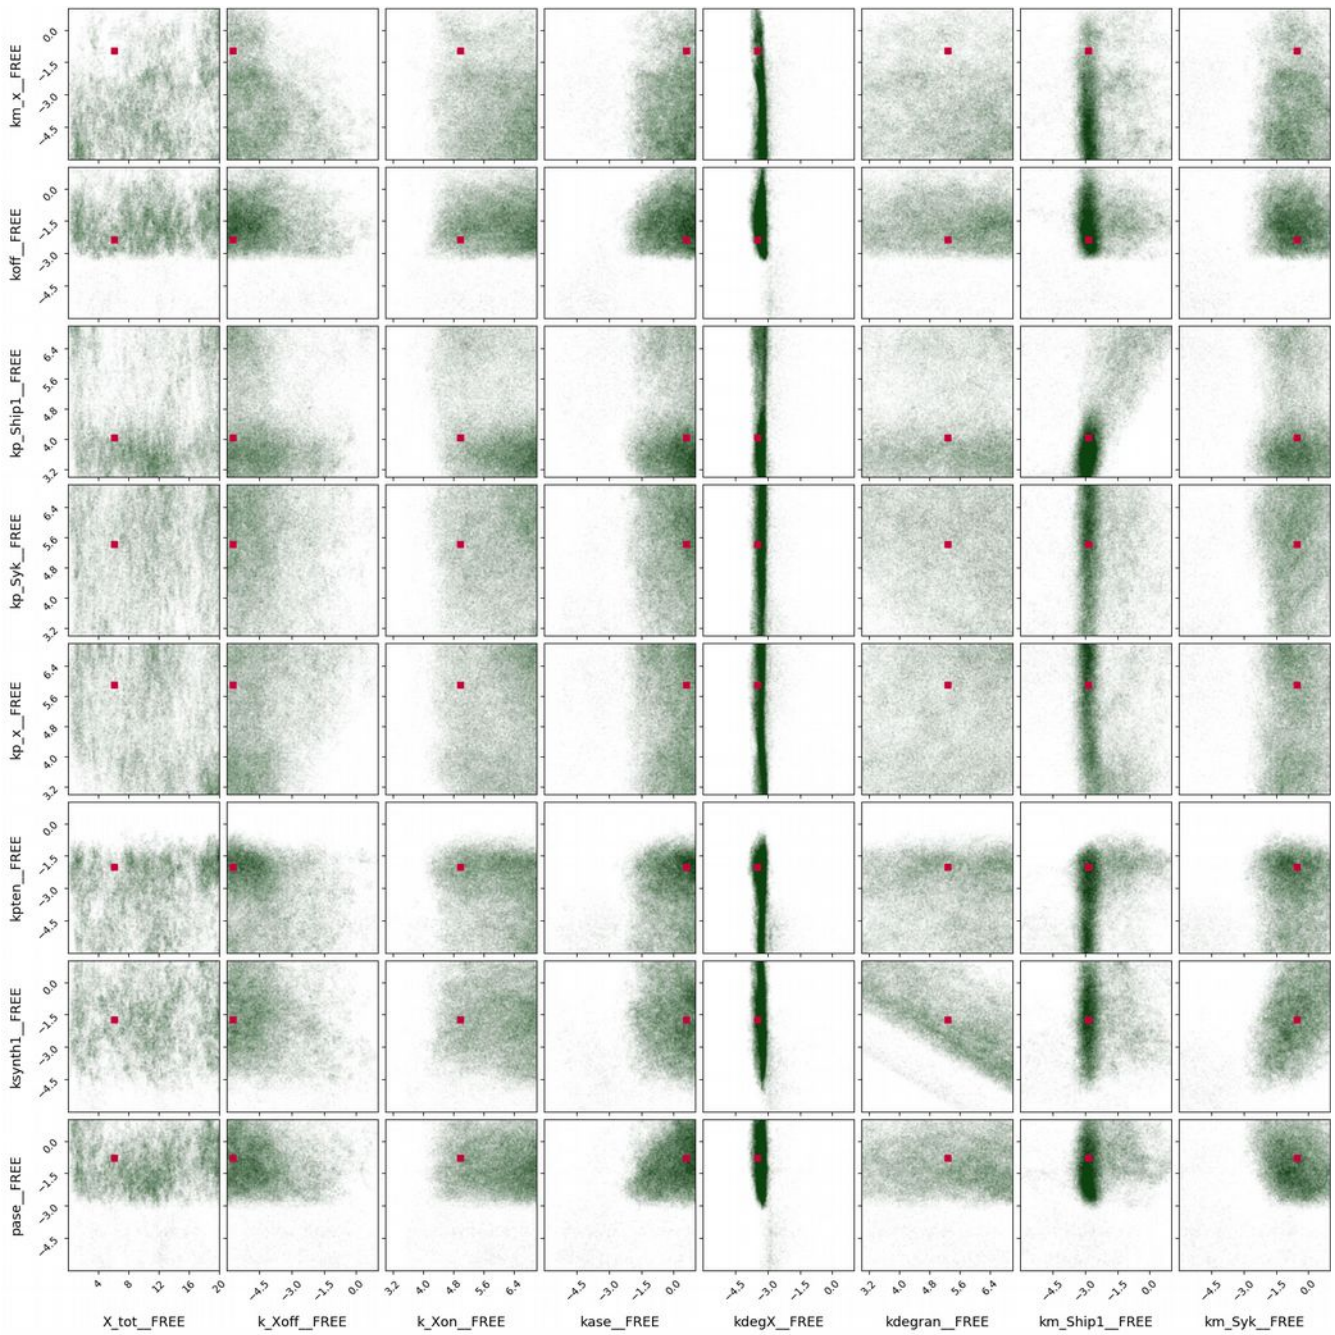


Figure S10: Corner plot showing the marginal posterior distribution for each pair of model parameters, under a measurement protocol consisting of 64 qualitative measurements, each with three possible categorical outcomes. The plot is split over the previous three pages for display purposes. Ground truth parameters are shown in red.

6 quantitative measurements

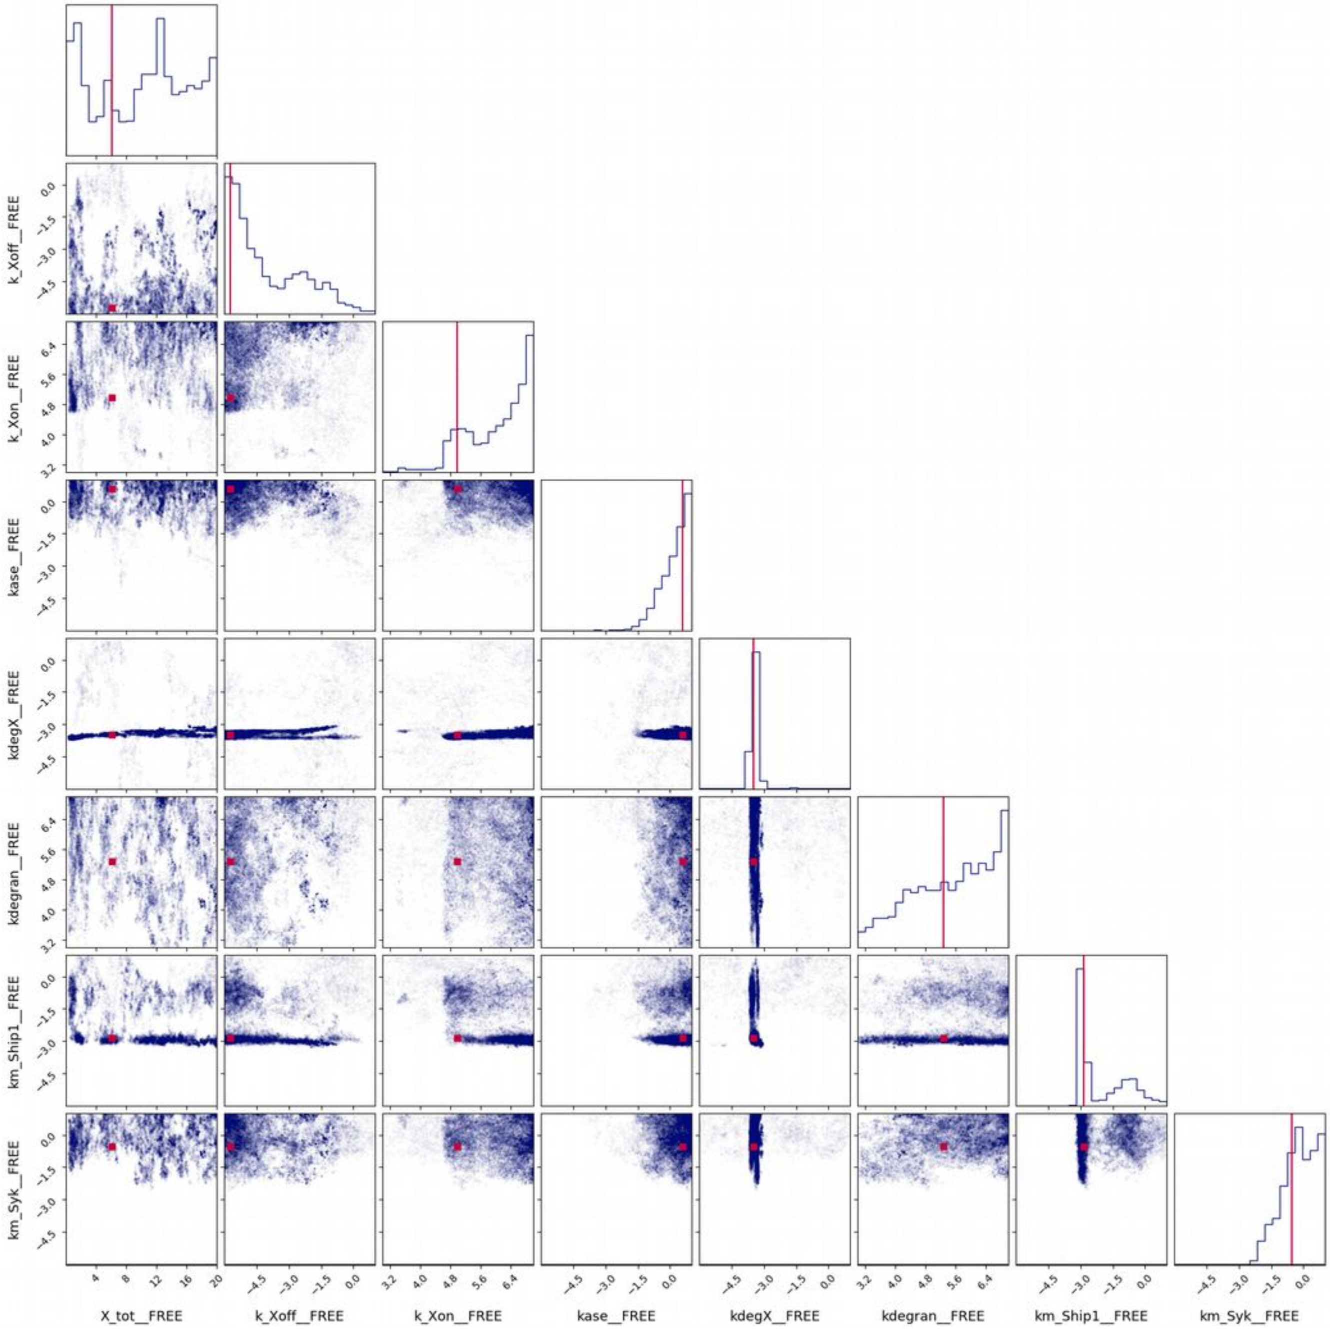

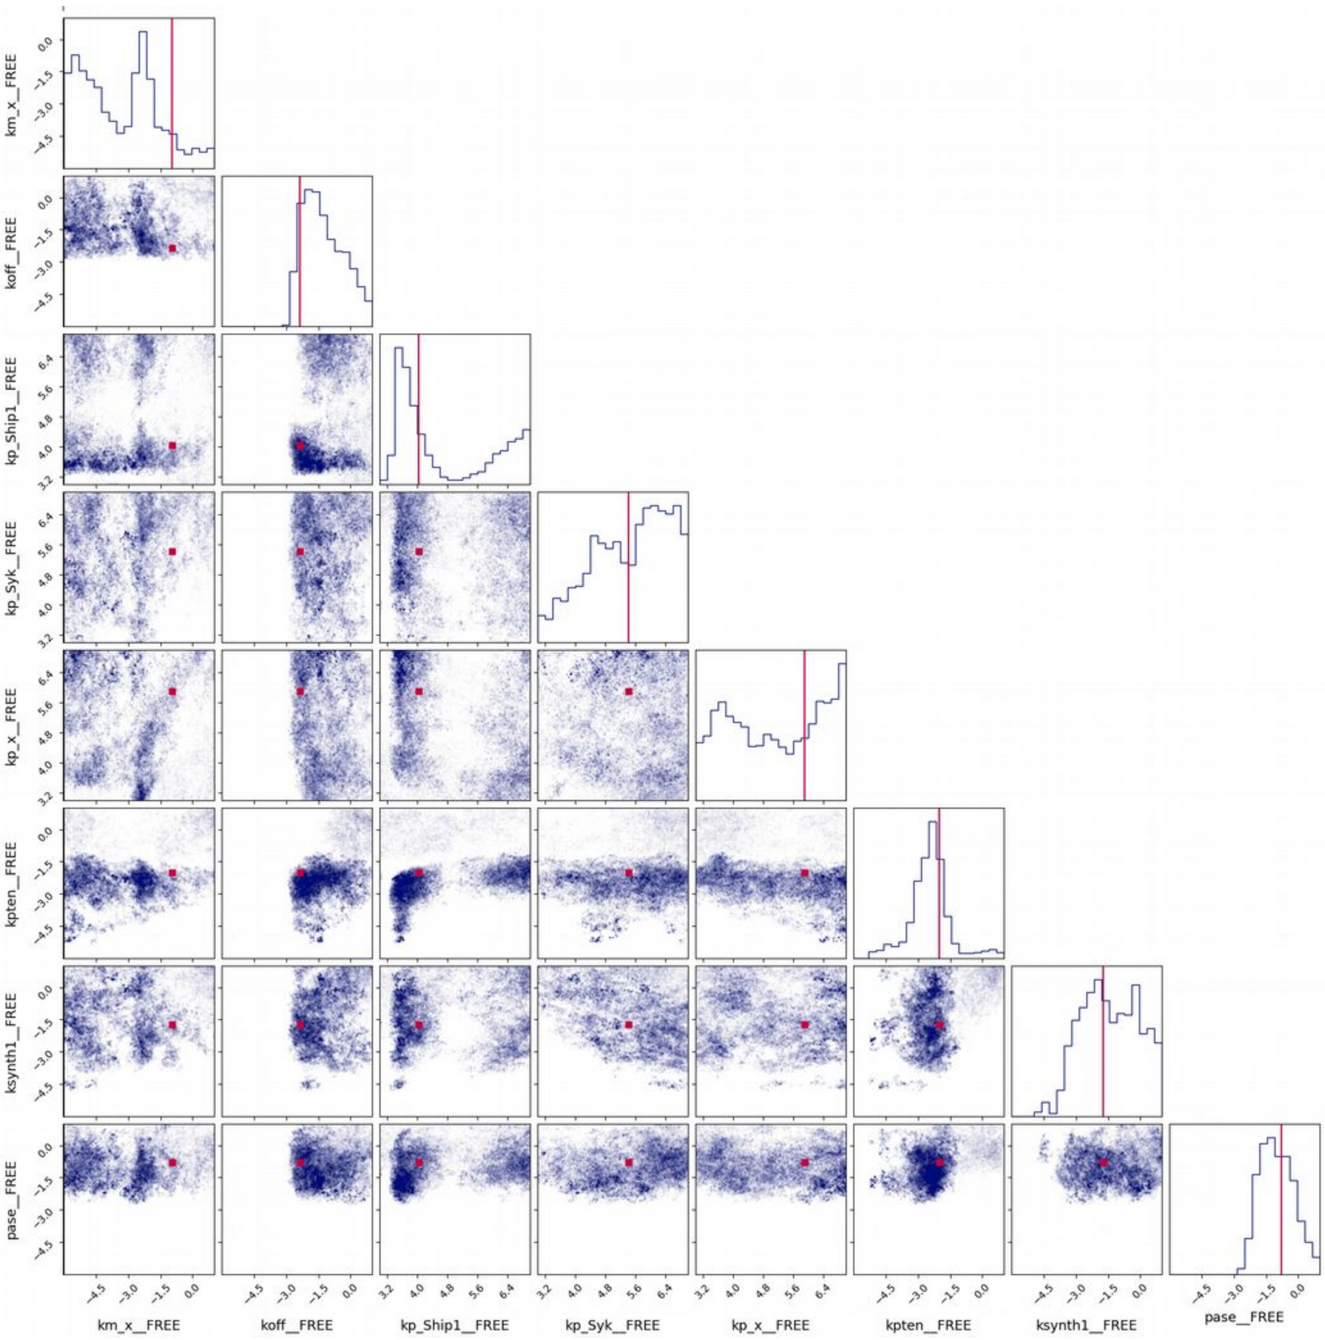
km_x__FREE
koff__FREE
kp_Ship1__FREE
kp_Syk__FREE
kp_x__FREE
kpten__FREE
ksynth1__FREE
pase__FREE

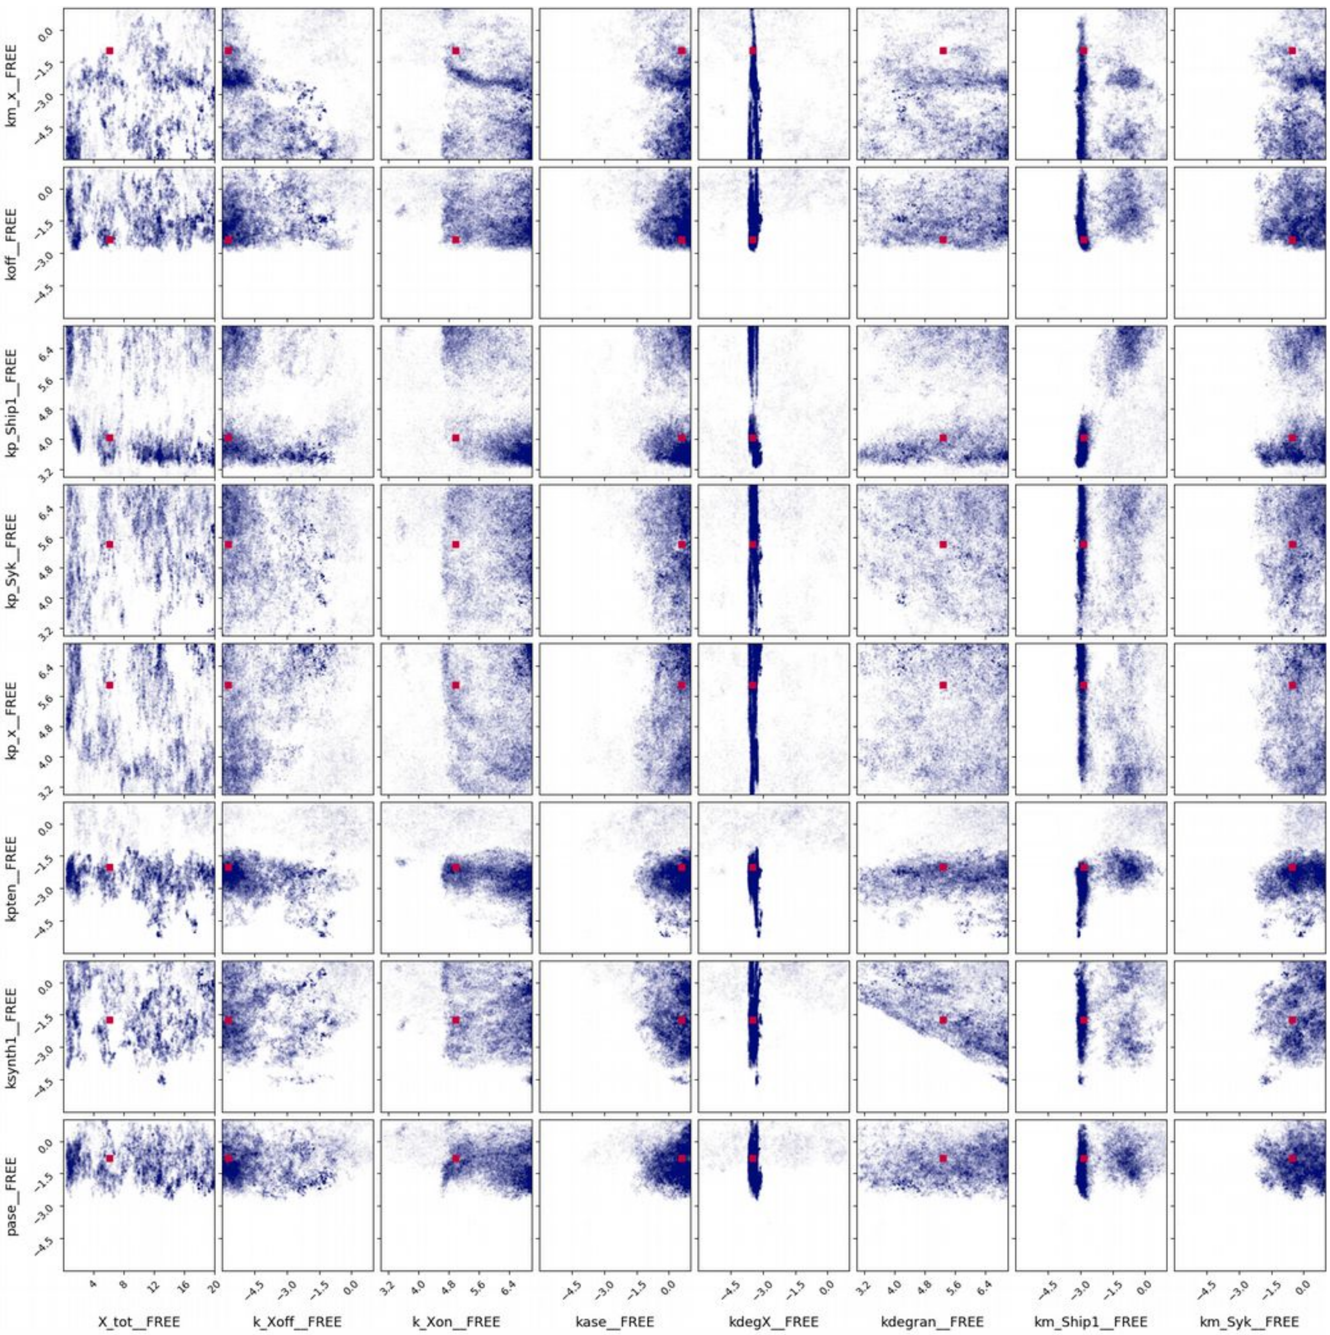


Figure S11: Corner plot showing the marginal posterior distribution for each pair of model parameters, under a measurement protocol consisting of six quantitative measurements. The plot is split over the previous three pages for display purposes. Ground truth parameters are shown in red.
